# Supplementary material for: Type I Planet Migration in a Magnetized Disk. II. Effect of Vertical Angular Momentum Transport
Source: arXiv:1501.02707 ancillary file (2015-01-12)
Supplement: Supplementary file 1 [file PaperIISup.pdf]

(\*\*\*\*\*

For Bans, Koenigl, & Uribe (2014):

This file provides the coefficients (A0 A1 A2 S0 S1) which govern the differential equation for the radial Lagrangian displacement, the numerical solution of which is critical for evaluating the torque exerted by the planet on the disk.

Here the field configuration is given by:  $B = \{0, D_b \phi z, b_z r^{nz}\}$ , where  $D_b \phi = B_{\phi 0} \left( = \frac{\partial B_{\phi 0}}{\partial \phi} \right)$ , as explained in Bans, Koenigl, and Uribe (2014). After evaluating the perturbed field and Lorentz force (Equations (14)-(15) in the aforementioned text) we vertically average by integrating from  $-H$  to  $H$ .

Other variable definitions:

- $k = k_z$  the vertical mode number,  $m$  is the azimuthal mode  
 $-\Sigma[r]$  is the surface density  
 $-\sigma[r]$  is the differential frequency,  $= \Omega - 1$   
 $-c[r]$  is the sound speed

\*\*\*\*\* )

$$A2 = \left( -b_z^2 D_b \phi^2 r^{2nz} \left( 3 b_z^2 H^2 k^2 r^{2+2nz} (m^2 + k^2 r^2) + D_b \phi^2 H^2 (H^2 m^2 - 3 r^2) (m^2 + k^2 r^2) - 3 i b_z D_b \phi m r^{1+nz} (-3 r^2 + H^2 (m^2 - k^2 r^2)) \right) + m^2 r^2 (-9 i b_z^3 D_b \phi m r^{1+3nz} + 9 b_z^4 k^2 r^{2+4nz} + D_b \phi^4 (H^4 m^2 - 3 H^2 r^2) + 3 b_z^2 D_b \phi^2 r^{2nz} (-3 r^2 + 2 H^2 (m^2 + k^2 r^2)) \right) \sigma[r]^2 \Sigma[r] - 3 m^4 r^4 (D_b \phi^2 H^2 + 3 b_z^2 r^{2nz}) \sigma[r]^4 \Sigma[r]^2 - c[r]^2 \Sigma[r] (-9 i b_z^3 D_b \phi k^2 m r^{3+3nz} + 9 b_z^4 k^4 r^{4+4nz} - 3 i b_z D_b \phi^3 m r^{1+nz} (H^2 m^2 - 3 r^2) + 3 b_z^2 D_b \phi^2 k^2 r^{2+2nz} (2 H^2 m^2 - 3 r^2) + D_b \phi^4 (H^4 m^4 - 3 H^2 m^2 r^2) - 3 m^2 r^2 (-3 i b_z D_b \phi m r^{1+nz} + 6 b_z^2 k^2 r^{2+2nz} + D_b \phi^2 (2 H^2 m^2 - 3 r^2)) \sigma[r]^2 \Sigma[r] + 9 m^4 r^4 \sigma[r]^4 \Sigma[r]^2) \right) / \left( 3 \Sigma[r] (b_z^2 D_b \phi^2 r^{2nz} (-3 m^2 r^2 + H^2 (m^2 + k^2 r^2)^2) - m^2 r^2 (3 b_z^2 r^{2nz} (m^2 + k^2 r^2) + D_b \phi^2 (-3 r^2 + H^2 (m^2 + k^2 r^2))) \sigma[r]^2 \Sigma[r] + 3 m^4 r^4 \sigma[r]^4 \Sigma[r]^2 + c[r]^2 \Sigma[r] (-6 i b_z D_b \phi k^2 m r^{3+nz} + 3 b_z^2 k^2 r^{2+2nz} (m^2 + k^2 r^2) + D_b \phi^2 m^2 (-3 r^2 + H^2 (m^2 + k^2 r^2)) - 3 m^2 r^2 (m^2 + k^2 r^2) \sigma[r]^2 \Sigma[r])) \right)$$

$$A1 = \left( -3 m r^2 K^2[r] \sigma[r] \Sigma[r]^2 \left( c[r]^4 \Sigma[r]^2 (9 b_z^4 k^4 m r^{4+4nz} (m^2 + k^2 r^2) - 9 i b_z^3 D_b \phi k^4 r^{5+3nz} (3 m^2 + k^2 r^2) + D_b \phi^4 m^3 (H^2 m^2 - 3 r^2) (-3 r^2 + H^2 (m^2 + k^2 r^2)) - 3 i b_z D_b \phi^3 k^2 m^2 r^{3+nz} (-9 r^2 + H^2 (3 m^2 + k^2 r^2)) + 3 b_z^2 D_b \phi^2 k^2 m r^{2+2nz} (-6 m^2 r^2 - 9 k^2 r^4 + 2 H^2 (m^4 + k^2 m^2 r^2)) \right) - 3 m^2 r^2 (6 b_z^2 k^2 m r^{2+2nz} (m^2 + k^2 r^2) - 3 i b_z D_b \phi k^2 r^{3+nz} (3 m^2 + k^2 r^2) + D_b \phi^2 (-3 m r^2 (2 m^2 + k^2 r^2) + 2 H^2 (m^5 + k^2 m^3 r^2))) \sigma[r]^2 \Sigma[r] + 9 m^5 r^4 (m^2 + k^2 r^2) \sigma[r]^4 \Sigma[r]^2 - c[r]^2 \Sigma[r] (b_z D_b \phi^3 r^{nz} (i D_b \phi^3 H^2 k^2 m^2 r^3 (-3 r^2 + H^2 (m^2 + k^2 r^2)) - 3 b_z^3 k^2 m r^{2+3nz} (2 H^2 (m^2 + k^2 r^2)^2 - 3 r^2 (2 m^2 + k^2 r^2)) + 3 i b_z^2 D_b \phi k^2 r^{3+2nz} (-9 m^2 r^2 + H^2 (3 m^4 + 5 k^2 m^2 r^2 + 2 k^4 r^4)) -$$

$$\begin{aligned}
& \text{bz Db}\phi^2 \text{ m r}^{nz} \left( 18 \text{ m}^2 \text{ r}^4 + 2 \text{ H}^4 \left( \text{m}^3 + \text{k}^2 \text{ m r}^2 \right)^2 - 3 \text{ H}^2 \left( 4 \text{ m}^4 \text{ r}^2 + 4 \text{ k}^2 \text{ m}^2 \text{ r}^4 + 3 \text{ k}^4 \text{ r}^6 \right) \right) + \\
& \text{m}^2 \text{ r}^2 \left( 18 \text{ bz}^4 \text{ k}^2 \text{ m r}^{2+4nz} \left( \text{m}^2 + \text{k}^2 \text{ r}^2 \right) - 9 \text{ i bz}^3 \text{ Db}\phi \text{ k}^2 \text{ r}^{3+3nz} \left( 3 \text{ m}^2 + \text{k}^2 \text{ r}^2 \right) + \right. \\
& \text{Db}\phi^4 \text{ m} \left( \text{H}^2 \text{ m}^2 - 3 \text{ r}^2 \right) \left( -3 \text{ r}^2 + \text{H}^2 \left( \text{m}^2 + \text{k}^2 \text{ r}^2 \right) \right) + 3 \text{ bz}^2 \text{ Db}\phi^2 \text{ m r}^{2nz} \left( 4 \text{ m}^2 + 3 \text{ k}^2 \text{ r}^2 \right) \\
& \left. \left( -3 \text{ r}^2 + \text{H}^2 \left( \text{m}^2 + \text{k}^2 \text{ r}^2 \right) \right) - 3 \text{ i bz Db}\phi^3 \text{ k}^2 \text{ r}^{3+nz} \left( -3 \text{ r}^2 + 2 \text{ H}^2 \left( \text{m}^2 + \text{k}^2 \text{ r}^2 \right) \right) \right) \sigma[\text{r}]^2 \Sigma[\text{r}] - \\
& 3 \text{ m}^4 \text{ r}^4 \left( -3 \text{ i bz Db}\phi \text{ k}^2 \text{ r}^{3+nz} + 3 \text{ bz}^2 \text{ m r}^{2nz} \left( 2 \text{ m}^2 + 3 \text{ k}^2 \text{ r}^2 \right) + \text{Db}\phi^2 \text{ m} \left( -6 \text{ r}^2 + \text{H}^2 \left( 2 \text{ m}^2 + \text{k}^2 \text{ r}^2 \right) \right) \right) \\
& \sigma[\text{r}]^4 \Sigma[\text{r}]^2 + 9 \text{ m}^7 \text{ r}^6 \sigma[\text{r}]^6 \Sigma[\text{r}]^3 + \text{bz r}^{nz} \\
& \left( \text{bz}^2 \text{ Db}\phi^4 \text{ r}^{2nz} \left( -3 \text{ m}^2 \text{ r}^2 + \text{H}^2 \left( \text{m}^2 + \text{k}^2 \text{ r}^2 \right)^2 \right) \left( -\text{i Db}\phi \text{ H}^2 \text{ k}^2 \text{ r}^3 + \text{bz m r}^{nz} \left( -3 \text{ r}^2 + \text{H}^2 \left( \text{m}^2 + \text{k}^2 \text{ r}^2 \right) \right) \right) + \right. \\
& \text{Db}\phi^2 \text{ m}^2 \text{ r}^2 \left( 3 \text{ i bz}^2 \text{ Db}\phi \text{ H}^2 \text{ k}^2 \text{ r}^{3+2nz} \left( \text{m}^2 + \text{k}^2 \text{ r}^2 \right) + \right. \\
& \text{i Db}\phi^3 \text{ H}^2 \text{ k}^2 \text{ r}^3 \left( -3 \text{ r}^2 + \text{H}^2 \left( \text{m}^2 + \text{k}^2 \text{ r}^2 \right) \right) - \text{bz Db}\phi^2 \text{ m r}^{nz} \left( -3 \text{ r}^2 + \text{H}^2 \left( \text{m}^2 + \text{k}^2 \text{ r}^2 \right) \right)^2 - \\
& 3 \text{ bz}^3 \text{ m r}^{3nz} \left( 2 \text{ H}^2 \left( \text{m}^2 + \text{k}^2 \text{ r}^2 \right)^2 - 3 \text{ r}^2 \left( 2 \text{ m}^2 + \text{k}^2 \text{ r}^2 \right) \right) \sigma[\text{r}]^2 \Sigma[\text{r}] + \\
& 3 \text{ m}^4 \text{ r}^4 \left( -\text{i Db}\phi^3 \text{ H}^2 \text{ k}^2 \text{ r}^3 + 3 \text{ bz}^3 \text{ m r}^{3nz} \left( \text{m}^2 + \text{k}^2 \text{ r}^2 \right) + 2 \text{ bz Db}\phi^2 \text{ m r}^{nz} \left( -3 \text{ r}^2 + \text{H}^2 \left( \text{m}^2 + \text{k}^2 \text{ r}^2 \right) \right) \right) \\
& \left. \sigma[\text{r}]^4 \Sigma[\text{r}]^2 - 9 \text{ bz m}^7 \text{ r}^{6+nz} \sigma[\text{r}]^6 \Sigma[\text{r}]^3 \right) + \\
& 2 \Omega[\text{r}] \left( -3 \text{ i bz}^4 \text{ Db}\phi^5 \text{ r}^{2+4nz} \left( -3 \text{ m}^2 \text{ r}^2 + \text{H}^2 \left( \text{m}^2 + \text{k}^2 \text{ r}^2 \right)^2 \right) \left( -\text{i Db}\phi \text{ H}^2 \text{ k}^2 \text{ r}^3 + \right. \right. \\
& \left. \left. \text{bz m r}^{nz} \left( -3 \text{ r}^2 + \text{H}^2 \left( \text{m}^2 + \text{k}^2 \text{ r}^2 \right) \right) \right) \Sigma'[\text{r}] - \text{bz}^2 \text{ Db}\phi^2 \text{ r}^{2nz} \Sigma[\text{r}] \right. \\
& \left. \left( \text{bz Db}\phi^2 \text{ r}^{nz} \left( 3 \text{ bz}^3 \text{ k}^2 \text{ r}^{2+3nz} \left( -9 \text{ m}^2 \text{ nz r}^4 + \text{H}^4 \left( \text{m}^2 + \text{k}^2 \text{ r}^2 \right)^2 \left( \text{m}^2 \left( 3 + 2 \text{ nz} \right) + \text{k}^2 \left( 1 + 2 \text{ nz} \right) \text{ r}^2 \right) - \right. \right. \right. \right. \\
& \left. \left. 3 \text{ H}^2 \text{ r}^2 \left( \text{m}^4 \left( 1 + \text{nz} \right) + 3 \text{ k}^2 \text{ m}^2 \text{ r}^2 - \text{k}^4 \text{ nz r}^4 \right) \right) - 3 \text{ i bz}^2 \text{ Db}\phi \text{ m r}^{1+2nz} \right. \\
& \left. \left( 9 \text{ m}^2 \left( 1 + \text{nz} \right) \text{ r}^4 - 3 \text{ H}^2 \text{ r}^2 \left( 2 \text{ m}^4 \left( 1 + \text{nz} \right) + \text{k}^2 \text{ m}^2 \left( -1 + \text{nz} \right) \text{ r}^2 + \text{k}^4 \left( -1 + \text{nz} \right) \text{ r}^4 \right) + \right. \right. \\
& \left. \left. \text{H}^4 \left( \text{m}^2 + \text{k}^2 \text{ r}^2 \right) \left( \text{m}^4 \left( 1 + \text{nz} \right) - 8 \text{ k}^2 \text{ m}^2 \text{ r}^2 - \text{k}^4 \left( 1 + \text{nz} \right) \text{ r}^4 \right) \right) + \right. \\
& \text{i Db}\phi^3 \text{ H}^2 \text{ m r} \left( 9 \text{ m}^2 \text{ r}^4 + \text{H}^4 \left( \text{m}^2 + \text{k}^2 \text{ r}^2 \right)^3 - 3 \text{ H}^2 \left( 2 \text{ m}^4 \text{ r}^2 + 3 \text{ k}^2 \text{ m}^2 \text{ r}^4 + \text{k}^4 \text{ r}^6 \right) \right) - \\
& \text{bz Db}\phi^2 \text{ H}^2 \text{ r}^{nz} \left( -\text{H}^4 \left( \text{m}^2 - \text{k}^2 \text{ r}^2 \right) \left( \text{m}^3 + \text{k}^2 \text{ m r}^2 \right)^2 - 9 \text{ m}^2 \text{ r}^4 \left( \text{m}^2 + \text{k}^2 \left( 3 + \text{nz} \right) \text{ r}^2 \right) + \right. \\
& \left. 3 \text{ H}^2 \left( 2 \text{ m}^6 \text{ r}^2 + \text{k}^2 \text{ m}^4 \left( 8 + \text{nz} \right) \text{ r}^4 + \text{k}^4 \text{ m}^2 \left( 5 + 2 \text{ nz} \right) \text{ r}^6 + \text{k}^6 \left( 1 + \text{nz} \right) \text{ r}^8 \right) \right) + \\
& 3 \text{ r}^2 \left( -9 \text{ bz}^4 \text{ k}^4 \text{ m}^2 \text{ r}^{5+4nz} + 6 \text{ i bz}^3 \text{ Db}\phi \text{ k}^2 \text{ m r}^{2+3nz} \left( \text{m}^2 + \text{k}^2 \text{ r}^2 \right) \left( -3 \text{ r}^2 + \text{H}^2 \left( \text{m}^2 + \text{k}^2 \text{ r}^2 \right) \right) + \right. \\
& \text{Db}\phi^4 \text{ H}^2 \text{ k}^2 \text{ m}^2 \text{ r}^3 \left( -6 \text{ r}^2 + \text{H}^2 \left( 2 \text{ m}^2 + \text{k}^2 \text{ r}^2 \right) \right) + 3 \text{ bz}^2 \text{ Db}\phi^2 \text{ k}^2 \text{ r}^{3+2nz} \\
& \left. \left( -15 \text{ m}^2 \text{ r}^2 + \text{H}^2 \left( 5 \text{ m}^4 + 6 \text{ k}^2 \text{ m}^2 \text{ r}^2 + 3 \text{ k}^4 \text{ r}^4 \right) \right) + \text{i bz Db}\phi^3 \text{ m r}^{nz} \left( 27 \text{ m}^2 \text{ r}^4 + \right. \right. \\
& \left. \left. \text{H}^4 \left( \text{m}^2 + \text{k}^2 \text{ r}^2 \right)^2 \left( 3 \text{ m}^2 + \text{k}^2 \text{ r}^2 \right) - 3 \text{ H}^2 \left( 6 \text{ m}^4 \text{ r}^2 + 7 \text{ k}^2 \text{ m}^2 \text{ r}^4 + 5 \text{ k}^4 \text{ r}^6 \right) \right) \right) \text{c}[\text{r}]^2 \Sigma'[\text{r}] - \\
& 3 \text{ m}^2 \text{ r}^3 \left( -9 \text{ bz}^4 \text{ k}^2 \text{ m}^2 \text{ r}^{4+4nz} + 6 \text{ i bz}^3 \text{ Db}\phi \text{ m r}^{1+3nz} \left( \text{H}^2 \text{ m}^2 - 3 \text{ r}^2 \right) \left( \text{m}^2 + \text{k}^2 \text{ r}^2 \right) + 2 \text{ i bz Db}\phi^3 \right. \\
& \left. \text{m r}^{1+nz} \left( \text{H}^2 \text{ m}^2 - 3 \text{ r}^2 \right) \left( -3 \text{ r}^2 + \text{H}^2 \left( \text{m}^2 + \text{k}^2 \text{ r}^2 \right) \right) + \text{Db}\phi^4 \text{ H}^2 \text{ k}^2 \text{ r}^4 \left( -6 \text{ r}^2 + \text{H}^2 \left( 2 \text{ m}^2 + \text{k}^2 \text{ r}^2 \right) \right) + \right. \\
& \left. \text{bz}^2 \text{ Db}\phi^2 \text{ r}^{2nz} \left( 9 \text{ m}^2 \text{ r}^4 + \text{H}^4 \left( \text{m}^2 + \text{k}^2 \text{ r}^2 \right)^3 + \text{H}^2 \left( -6 \text{ m}^4 \text{ r}^2 + 6 \text{ k}^4 \text{ r}^6 \right) \right) \right) \sigma[\text{r}]^2 \Sigma'[\text{r}] + \\
& 3 \text{ m r}^2 \sigma[\text{r}] \Sigma[\text{r}]^4 \left( -2 \text{ m}^3 \text{ r}^3 \left( 9 \text{ i bz}^3 \text{ Db}\phi \text{ k}^2 \text{ m r}^{3+3nz} + 9 \text{ bz}^4 \text{ k}^4 \text{ r}^{4+4nz} + 3 \text{ bz}^2 \text{ Db}\phi^2 \text{ k}^2 \text{ r}^{2+2nz} \right. \right. \\
& \left. \left. \left( 2 \text{ H}^2 \text{ m}^2 - 9 \text{ r}^2 \right) + \text{Db}\phi^4 \left( \text{H}^2 \text{ m}^2 - 3 \text{ r}^2 \right)^2 - 3 \text{ i bz Db}\phi^3 \text{ m r}^{1+nz} \left( -6 \text{ r}^2 + \text{H}^2 \left( 2 \text{ m}^2 - \text{k}^2 \text{ r}^2 \right) \right) \right) \right) \\
& \text{c}[\text{r}] \sigma[\text{r}]^3 \text{c}'[\text{r}] + \text{m}^4 \text{ r}^4 \sigma[\text{r}]^4 \left( \text{m} \left( 3 \text{ i bz Db}\phi^3 \text{ H}^2 \text{ m r}^{1+nz} - 9 \text{ i bz}^3 \text{ Db}\phi \text{ m} \right. \right. \\
& \left. \left. \left( -1 + 3 \text{ nz} \right) \text{ r}^{1+3nz} + 9 \text{ bz}^4 \text{ r}^{4nz} \left( 3 \text{ m}^2 + 2 \text{ k}^2 \left( 1 + 2 \text{ nz} \right) \text{ r}^2 \right) + 6 \text{ bz}^2 \text{ Db}\phi^2 \text{ r}^{2nz} \right. \right. \\
& \left. \left. \left( -3 \left( 1 + 2 \text{ nz} \right) \text{ r}^2 + 2 \text{ H}^2 \left( 1 + \text{nz} \right) \left( \text{m}^2 + \text{k}^2 \text{ r}^2 \right) \right) + \text{Db}\phi^4 \left( -6 \text{ H}^2 \text{ r}^2 + \text{H}^4 \left( 2 \text{ m}^2 + \text{k}^2 \text{ r}^2 \right) \right) \right) \right) \\
& \sigma[\text{r}] + 6 \text{ bz r}^{nz} \left( 3 \text{ bz}^3 \text{ m r}^{3nz} \left( \text{m}^2 + \text{k}^2 \text{ r}^2 \right) + 3 \text{ i bz}^2 \text{ Db}\phi \text{ r}^{1+2nz} \left( \text{m}^2 + \text{k}^2 \text{ r}^2 \right) + \right. \\
& \left. 2 \text{ bz Db}\phi^2 \text{ m r}^{nz} \left( -3 \text{ r}^2 + \text{H}^2 \left( \text{m}^2 + \text{k}^2 \text{ r}^2 \right) \right) + \text{i Db}\phi^3 \left( -6 \text{ r}^3 + \text{H}^2 \left( 2 \text{ m}^2 \text{ r} + \text{k}^2 \text{ r}^3 \right) \right) \right) \Omega[\text{r}] + \\
& \text{r} \left( 2 \text{ Db}\phi^4 \text{ H}^4 \text{ k}^2 \text{ m r}^2 - 3 \text{ i bz Db}\phi^3 \text{ H}^2 \text{ k}^2 \text{ r}^{3+nz} + 18 \text{ i bz}^3 \text{ Db}\phi \text{ m}^2 \text{ r}^{1+3nz} + \right. \\
& \left. 9 \text{ bz}^4 \text{ m r}^{4nz} \left( 3 \text{ m}^2 + \text{k}^2 \text{ r}^2 \right) + 6 \text{ bz}^2 \text{ Db}\phi^2 \text{ m r}^{2nz} \left( -3 \text{ r}^2 + \text{H}^2 \left( \text{m}^2 + \text{k}^2 \text{ r}^2 \right) \right) \right) \Omega'[\text{r}] + \\
& \text{c}[\text{r}]^4 \left( \text{m} \left( -18 \text{ i bz}^3 \text{ Db}\phi \text{ k}^2 \text{ m r}^{3+3nz} \left( \text{m}^2 \left( 1 + 2 \text{ nz} \right) + \text{k}^2 \left( 3 + 4 \text{ nz} \right) \text{ r}^2 \right) + \right. \right. \\
& \left. \left. 9 \text{ bz}^4 \text{ k}^4 \text{ r}^{4+4nz} \left( \text{m}^2 \left( 9 + 4 \text{ nz} \right) + \text{k}^2 \left( 3 + 4 \text{ nz} \right) \text{ r}^2 \right) + 3 \text{ bz}^2 \text{ Db}\phi^2 \text{ k}^2 \text{ r}^{2+2nz} \right. \right. \\
& \left. \left. \left( -3 \text{ r}^2 \left( \text{m}^2 \left( 11 + 7 \text{ nz} \right) + \text{k}^2 \left( 1 + \text{nz} \right) \text{ r}^2 \right) + 2 \text{ H}^2 \text{ m}^2 \left( \text{m}^2 \left( 7 + 2 \text{ nz} \right) + \text{k}^2 \left( 1 + 2 \text{ nz} \right) \text{ r}^2 \right) \right) + \right. \right. \\
& \left. \left. \text{Db}\phi^4 \text{ m}^2 \left( 27 \text{ r}^4 + \text{H}^4 \left( 5 \text{ m}^4 - \text{k}^2 \text{ m}^2 \text{ r}^2 \right) - 6 \text{ H}^2 \left( 4 \text{ m}^2 \text{ r}^2 + \text{k}^2 \text{ r}^4 \right) \right) - 3 \text{ i bz Db}\phi^3 \text{ m r}^{1+nz} \right. \right. \\
& \left. \left. \left( -3 \text{ r}^2 \left( \text{m}^2 \left( 2 + 4 \text{ nz} \right) + 3 \text{ k}^2 \text{ r}^2 \right) + 2 \text{ H}^2 \left( \text{m}^4 \left( 1 + 2 \text{ nz} \right) - 2 \text{ k}^2 \text{ m}^2 \text{ r}^2 - \text{k}^4 \text{ r}^4 \right) \right) \right) \right) \sigma[\text{r}] + \\
& 2 \text{ m} \left( -18 \text{ i bz}^3 \text{ Db}\phi \text{ k}^4 \text{ m r}^{5+3nz} - 6 \text{ i bz Db}\phi^3 \text{ k}^2 \text{ m r}^{3+nz} \left( \text{H}^2 \text{ m}^2 - 3 \text{ r}^2 \right) + \right. \\
& \left. 9 \text{ bz}^4 \text{ k}^4 \text{ r}^{4+4nz} \left( \text{m}^2 + \text{k}^2 \text{ r}^2 \right) + \text{Db}\phi^4 \text{ m}^2 \left( \text{H}^2 \text{ m}^2 - 3 \text{ r}^2 \right) \left( -3 \text{ r}^2 + \text{H}^2 \left( \text{m}^2 + \text{k}^2 \text{ r}^2 \right) \right) + \right. \\
& \left. 3 \text{ bz}^2 \text{ Db}\phi^2 \text{ k}^2 \text{ r}^{2+2nz} \left( -3 \text{ r}^2 \left( 2 \text{ m}^2 + \text{k}^2 \text{ r}^2 \right) + 2 \text{ H}^2 \left( \text{m}^4 + \text{k}^2 \text{ m}^2 \text{ r}^2 \right) \right) \right) \Omega[\text{r}] -
\end{aligned}$$

$$\begin{aligned}
& 6 m^3 r^3 \left( 3 \, i \, b z \, D b \phi \, m \, r^{1+n z} \left( m^2 - k^2 r^2 \right) + 3 \, b z^2 k^2 r^{2+2 n z} \left( m^2 + k^2 r^2 \right) + \right. \\
& \quad D b \phi^2 m^2 \left( -3 r^2 + H^2 \left( m^2 + k^2 r^2 \right) \right) \sigma[r]^3 \Sigma'[r] + 3 r \left( 9 \, b z^4 k^4 m r^{4+4 n z} \left( m^2 + k^2 r^2 \right) - 3 \, i \, b z^3 \, D b \phi k^4 r^{5+3 n z} \left( 11 m^2 + k^2 r^2 \right) - i \, b z \, D b \phi^3 k^2 m^2 r^{3+n z} \left( -15 r^2 + H^2 \left( 11 m^2 + k^2 r^2 \right) \right) + \\
& \quad 3 \, b z^2 \, D b \phi^2 k^2 m r^{2+2 n z} \left( -10 m^2 r^2 - 3 k^2 r^4 + 2 H^2 \left( m^4 + k^2 m^2 r^2 \right) \right) + \\
& \quad \left. D b \phi^4 m^3 \left( 9 r^4 + H^4 \left( m^4 + k^2 m^2 r^2 \right) - H^2 \left( 6 m^2 r^2 + k^2 r^4 \right) \right) \right) \Omega'[r] - \\
& m^2 r^2 c[r]^2 \sigma[r]^2 \left( m \left( -3 \, i \, b z \, D b \phi^3 m r^{1+n z} \left( H^2 m^2 \left( -3 + 4 n z \right) + 6 \left( 1 - 2 n z \right) r^2 \right) + \right. \right. \\
& \quad 9 \, b z^4 k^2 r^{2+4 n z} \left( 4 m^2 \left( 3 + n z \right) + k^2 \left( 5 + 8 n z \right) r^2 \right) - 9 \, i \, b z^3 \, D b \phi m r^{1+3 n z} \\
& \quad \left( m^2 \left( 2 + 3 n z \right) + k^2 \left( 1 + 9 n z \right) r^2 \right) + D b \phi^4 \left( 5 H^4 m^4 + 9 r^4 - 6 H^2 \left( 3 m^2 r^2 + k^2 r^4 \right) \right) + \\
& \quad \left. 3 \, b z^2 \, D b \phi^2 r^{2 n z} \left( 2 H^2 \left( 7 m^4 + k^2 m^2 \left( 9 + 4 n z \right) r^2 + k^4 \left( 3 + 2 n z \right) r^4 \right) - \right. \right. \\
& \quad \left. \left. 3 \left( 12 m^2 r^2 + k^2 \left( 4 + 7 n z \right) r^4 \right) \right) \right) \sigma[r] + 2 \left( 9 \, i \, b z^3 \, D b \phi k^2 r^{3+3 n z} \left( -m^2 + k^2 r^2 \right) + \right. \\
& \quad 18 \, b z^4 k^2 m r^{2+4 n z} \left( m^2 + k^2 r^2 \right) + D b \phi^4 m \left( H^2 m^2 - 3 r^2 \right) \left( -3 r^2 + H^2 \left( m^2 + k^2 r^2 \right) \right) + \\
& \quad 3 \, i \, b z \, D b \phi^3 r^{1+n z} \left( -3 r^2 \left( 2 m^2 + k^2 r^2 \right) + 2 H^2 \left( m^4 + k^2 m^2 r^2 \right) \right) + \\
& \quad \left. 3 \, b z^2 \, D b \phi^2 m r^{2 n z} \left( -3 \left( 4 m^2 r^2 + k^2 r^4 \right) + H^2 \left( 4 m^4 + 7 k^2 m^2 r^2 + 3 k^4 r^4 \right) \right) \right) \Omega[r] - \\
& 6 m^3 r^3 \left( 3 \, i \, b z \, D b \phi m r^{1+n z} + 3 \, b z^2 r^{2 n z} \left( m^2 + k^2 r^2 \right) + D b \phi^2 \left( -3 r^2 + H^2 \left( m^2 + k^2 r^2 \right) \right) \right) \\
& \sigma[r]^3 \Sigma'[r] + r \left( 18 \, b z^4 k^2 m r^{2+4 n z} \left( 3 m^2 + k^2 r^2 \right) - 9 \, i \, b z^3 \, D b \phi k^2 r^{3+3 n z} \left( 7 m^2 + k^2 r^2 \right) + \right. \\
& \quad D b \phi^4 m \left( 9 r^4 + H^4 \left( m^4 + 5 k^2 m^2 r^2 \right) - 3 H^2 \left( 2 m^2 r^2 + k^2 r^4 \right) \right) - \\
& \quad \left. 3 \, i \, b z \, D b \phi^3 r^{1+n z} \left( 12 m^2 r^2 - 3 k^2 r^4 + 2 H^2 \left( -2 m^4 + 5 k^2 m^2 r^2 + k^4 r^4 \right) \right) + \right. \\
& \quad \left. \left. 3 \, b z^2 \, D b \phi^2 m r^{2 n z} \left( -36 m^2 r^2 + 3 k^2 r^4 + H^2 \left( 12 m^4 + 15 k^2 m^2 r^2 + 11 k^4 r^4 \right) \right) \right) \right) \Omega'[r] \Big) - \\
& 27 m^6 r^6 c[r] \sigma[r]^5 \Sigma[r]^6 \left( 2 m^2 r^3 \sigma[r]^3 c'[r] + m^2 r^2 c[r] \sigma[r]^2 \left( \sigma[r] + 2 \Omega[r] + r \Omega'[r] \right) - \right. \\
& \quad \left. c[r]^3 \left( \left( 3 m^2 + k^2 r^2 \right) \sigma[r] + \left( m^2 + k^2 r^2 \right) \left( 2 \Omega[r] + 3 r \Omega'[r] \right) \right) \right) - 9 m^3 r^4 \sigma[r]^3 \Sigma[r]^5 \\
& \left( -2 m^3 r^3 \left( -3 \, i \, b z \, D b \phi m r^{1+n z} + 6 \, b z^2 k^2 r^{2+2 n z} + 2 \, D b \phi^2 \left( H^2 m^2 - 3 r^2 \right) \right) c[r] \sigma[r]^3 c'[r] - \right. \\
& \quad m^2 r^2 c[r]^2 \sigma[r]^2 \left( m \left( -3 \, i \, b z \, D b \phi m \left( -1 + 2 n z \right) r^{1+n z} + 6 \, b z^2 r^{2 n z} \left( 3 m^2 + 2 k^2 \left( 1 + n z \right) r^2 \right) + \right. \right. \\
& \quad \left. \left. 2 \, D b \phi^2 \left( -3 r^2 + H^2 \left( 2 m^2 + k^2 r^2 \right) \right) \right) \right) \sigma[r] + 2 \left( 3 \, i \, b z \, D b \phi r^{1+n z} \left( m^2 + k^2 r^2 \right) + \right. \\
& \quad \left. 3 \, b z^2 m r^{2 n z} \left( 2 m^2 + 3 k^2 r^2 \right) + D b \phi^2 m \left( -6 r^2 + H^2 \left( 2 m^2 + k^2 r^2 \right) \right) \right) \Omega[r] - \\
& \quad \left. 3 m^3 r^3 \sigma[r]^3 \Sigma'[r] + r \left( -3 \, i \, b z \, D b \phi r^{1+n z} \left( -2 m^2 + k^2 r^2 \right) + 9 \, b z^2 m r^{2 n z} \right. \right. \\
& \quad \left. \left. \left( 2 m^2 + k^2 r^2 \right) + D b \phi^2 m \left( -6 r^2 + H^2 \left( 2 m^2 + 5 k^2 r^2 \right) \right) \right) \right) \Omega'[r] + \\
& c[r]^4 \left( m \left( -3 \, i \, b z \, D b \phi m r^{1+n z} \left( m^2 \left( 1 + 2 n z \right) + 3 k^2 r^2 \right) + 3 \, b z^2 k^2 r^{2+2 n z} \right. \right. \\
& \quad \left. \left( m^2 \left( 9 + 2 n z \right) + k^2 \left( 3 + 2 n z \right) r^2 \right) + D b \phi^2 \left( H^2 \left( 7 m^4 + k^2 m^2 r^2 \right) - 3 \left( 6 m^2 r^2 + k^2 r^4 \right) \right) \right) \right) \\
& \sigma[r] + 2 m \left( -6 \, i \, b z \, D b \phi k^2 m r^{3+n z} + 6 \, b z^2 k^2 r^{2+2 n z} \left( m^2 + k^2 r^2 \right) + D b \phi^2 \right. \\
& \quad \left. \left( -3 r^2 \left( 2 m^2 + k^2 r^2 \right) + 2 H^2 \left( m^4 + k^2 m^2 r^2 \right) \right) \right) \Omega[r] - 3 m^3 r^3 \left( m^2 + k^2 r^2 \right) \sigma[r]^3 \Sigma'[r] + \\
& \quad 3 r \left( 6 \, b z^2 k^2 m r^{2+2 n z} \left( m^2 + k^2 r^2 \right) - i \, b z \, D b \phi k^2 r^{3+n z} \left( 11 m^2 + k^2 r^2 \right) + \right. \\
& \quad \left. D b \phi^2 \left( -m r^2 \left( 6 m^2 + k^2 r^2 \right) + 2 H^2 \left( m^5 + k^2 m^3 r^2 \right) \right) \right) \Omega'[r] + \\
& m^4 r^4 \sigma[r]^4 \left( m \left( D b \phi^2 H^2 + 3 \, b z^2 \left( 1 + 2 n z \right) r^{2 n z} \right) \sigma[r] + 3 \, b z r^{n z} \right. \\
& \quad \left. \left( 2 \left( i \, D b \phi r + b z m r^{n z} \right) \Omega[r] + b z m r^{1+n z} \Omega'[r] \right) \right) - \\
& \Sigma[r]^3 \left( 6 \, b z \, D b \phi m^2 r^{4+n z} \left( -9 \, b z \, D b \phi^3 k^2 r^{5+n z} - 18 \, i \, b z^4 k^4 m r^{4+4 n z} + 9 \, b z^3 \, D b \phi k^2 \right. \right. \\
& \quad \left. \left. r^{3+3 n z} \left( -m^2 + k^2 r^2 \right) + i \, D b \phi^4 m \left( H^2 m^2 - 3 r^2 \right) \left( -3 r^2 + H^2 \left( m^2 - k^2 r^2 \right) \right) - \right. \right. \\
& \quad \left. \left. 3 \, i \, b z^2 \, D b \phi^2 k^2 m r^{2+2 n z} \left( -3 r^2 + H^2 \left( m^2 + k^2 r^2 \right) \right) \right) \right) c[r] \sigma[r]^2 c'[r] + \\
& c[r]^4 \left( 27 \, b z^6 k^6 r^{6+6 n z} \left( m^2 \left( 3 + 2 n z \right) + k^2 \left( 1 + 2 n z \right) r^2 \right) - \right. \\
& \quad 27 \, i \, b z^5 \, D b \phi k^4 m r^{5+5 n z} \left( m^2 \left( 1 + 2 n z \right) + k^2 \left( 3 + 8 n z \right) r^2 \right) + \\
& \quad 3 \, b z^2 \, D b \phi^4 k^2 m^2 r^{2+2 n z} \left( 9 \left( 2 + 5 n z \right) r^4 - 3 H^2 r^2 \left( m^2 \left( 3 + 7 n z \right) + k^2 \left( -3 + n z \right) r^2 \right) + \right. \\
& \quad \left. H^4 m^2 \left( m^2 \left( 5 + 2 n z \right) + k^2 \left( -1 + 2 n z \right) r^2 \right) \right) + 9 \, b z^4 \, D b \phi^2 k^4 r^{4+4 n z} \\
& \quad \left( -3 r^2 \left( m^2 \left( 5 + 11 n z \right) + k^2 n z r^2 \right) + H^2 m^2 \left( m^2 \left( 7 + 4 n z \right) + k^2 \left( 1 + 4 n z \right) r^2 \right) \right) + \\
& \quad D b \phi^6 H^2 m^4 \left( 9 r^4 + H^4 \left( m^4 - k^2 m^2 r^2 \right) - 3 H^2 \left( 2 m^2 r^2 + k^2 r^4 \right) \right) - \\
& \quad 3 \, i \, b z \, D b \phi^5 m^3 r^{1+n z} \left( 9 \left( 1 + 2 n z \right) r^4 + 3 H^2 r^2 \left( -2 m^2 \left( 1 + 2 n z \right) + k^2 r^2 \right) + \right. \\
& \quad \left. H^4 \left( m^4 \left( 1 + 2 n z \right) - 7 k^2 m^2 r^2 - 2 k^4 r^4 \right) \right) + 9 \, i \, b z^3 \, D b \phi^3 k^2 m r^{3+3 n z} \left( 3 r^2 \left( m^2 \left( 2 + 4 n z \right) + \right. \right. \\
& \quad \left. \left. k^2 \left( 1 + 4 n z \right) r^2 \right) - 2 H^2 \left( m^4 \left( 1 + 2 n z \right) + 2 k^2 m^2 \left( -1 + 2 n z \right) r^2 - k^4 r^4 \right) \right) -
\end{aligned}$$

$$\begin{aligned}
& 3 m^2 r^3 \left( -9 i b z^3 D b \phi k^2 m r^{3+3 n z} \left( -3 m^2 + k^2 r^2 \right) + 9 b z^4 k^4 r^{4+4 n z} \left( m^2 + k^2 r^2 \right) + 6 b z^2 D b \phi^2 \right. \\
& \quad \left. k^2 r^{2+2 n z} \left( H^2 m^2 + 3 r^2 \right) \left( m^2 + k^2 r^2 \right) + D b \phi^4 \left( -6 H^2 m^4 r^2 + 9 m^2 r^4 + H^4 \left( m^6 + k^2 m^4 r^2 \right) \right) \right) + \\
& \quad 3 i b z D b \phi^3 m r^{1+n z} \left( -3 \left( 4 m^2 r^2 + k^2 r^4 \right) + H^2 \left( 4 m^4 + k^2 m^2 r^2 + k^4 r^4 \right) \right) \sigma[r]^2 \Sigma'[r] + \\
& \quad m^3 r^4 \sigma[r]^3 \left( m \left( -27 i b z^5 D b \phi m r^{1+5 n z} \left( m^2 (1+n z) + k^2 (-1+n z) r^2 \right) + \right. \right. \\
& \quad \left. \left. 27 b z^6 k^2 r^{2+6 n z} \left( m^2 (3+2 n z) + k^2 (1+2 n z) r^2 \right) - 27 i b z^3 D b \phi^3 m r^{1+3 n z} \right. \right. \\
& \quad \left. \left( 2 (1-3 n z) r^2 + H^2 \left( m^2 (-1+2 n z) - k^2 r^2 \right) \right) + 6 i b z D b \phi^5 H^2 m r^{1+n z} \right. \\
& \quad \left. \left( -3 r^2 + H^2 \left( m^2 + k^2 r^2 \right) \right) + 3 b z^2 D b \phi^4 r^{2 n z} \left( 9 (1+2 n z) r^4 + H^4 \left( m^2 + k^2 r^2 \right) \right. \right. \\
& \quad \left. \left. \left( m^2 (5+2 n z) + k^2 (3+2 n z) r^2 \right) - 3 H^2 r^2 \left( m^2 (6+4 n z) + k^2 (5+7 n z) r^2 \right) \right) \right. \\
& \quad \left. D b \phi^6 \left( 9 H^2 r^4 + H^6 \left( m^4 - k^2 m^2 r^2 \right) - 3 H^4 \left( 2 m^2 r^2 + k^2 r^4 \right) \right) + 9 b z^4 D b \phi^2 r^{4 n z} \right. \\
& \quad \left. \left( H^2 \left( m^2 + k^2 r^2 \right) \left( 7 m^2 + k^2 (5+8 n z) r^2 \right) - 3 \left( 6 m^2 r^2 + k^2 (2+3 n z) r^4 \right) \right) \right) \sigma[r] - \\
& \quad 3 m^3 r^3 \left( D b \phi^4 H^4 k^2 r^2 + 9 b z^4 m^2 r^{4 n z} + 18 i b z^3 D b \phi m r^{1+3 n z} \right) \sigma[r]^3 \Sigma'[r] + \\
& \quad 3 b z D b \phi^2 r^{n z} \left( 2 \left( i D b \phi^3 r \left( H^2 m^2 - 3 r^2 \right) \left( -3 r^2 + H^2 \left( m^2 + k^2 r^2 \right) \right) + \right. \right. \\
& \quad \left. \left. 3 i b z^2 D b \phi r^{1+2 n z} \left( 2 m^2 + k^2 r^2 \right) \left( -3 r^2 + H^2 \left( m^2 + k^2 r^2 \right) \right) + b z D b \phi^2 m r^{n z} \right. \right. \\
& \quad \left. \left. \left( -3 r^2 + H^2 \left( m^2 + k^2 r^2 \right) \right)^2 + 3 b z^3 m r^{3 n z} \left( 2 H^2 \left( m^2 + k^2 r^2 \right)^2 - 3 r^2 \left( 2 m^2 + k^2 r^2 \right) \right) \right) \right) \\
& \quad \Omega[r] + r \left( -i D b \phi^3 H^2 k^2 r^3 \left( -3 r^2 + H^2 \left( m^2 + k^2 r^2 \right) \right) + 3 b z^3 m r^{3 n z} \right. \\
& \quad \left. \left( -3 \left( 6 m^2 r^2 + k^2 r^4 \right) + 2 H^2 \left( 3 m^4 + 4 k^2 m^2 r^2 + k^4 r^4 \right) \right) - \right. \\
& \quad \left. 3 i b z^2 D b \phi r^{1+2 n z} \left( 12 m^2 r^2 + H^2 \left( -4 m^4 + 5 k^2 m^2 r^2 + k^4 r^4 \right) \right) + b z D b \phi^2 m \right. \\
& \quad \left. r^{n z} \left( 9 r^4 + H^2 \left( -6 m^2 r^2 + 6 k^2 r^4 \right) + H^4 \left( m^4 + 6 k^2 m^2 r^2 + 5 k^4 r^4 \right) \right) \right) \Omega'[r] \Big) + \\
& \quad m r^2 c[r]^2 \sigma[r] \left( -m \left( 54 b z^6 k^4 r^{4+6 n z} \left( m^2 (3+2 n z) + k^2 (1+2 n z) r^2 \right) - \right. \right. \\
& \quad \left. \left. 27 i b z^5 D b \phi k^2 m r^{3+5 n z} \left( m^2 (2+3 n z) + k^2 (2+9 n z) r^2 \right) + \right. \right. \\
& \quad \left. \left. 2 D b \phi^6 H^2 m^2 \left( 9 r^4 + H^4 \left( m^4 - k^2 m^2 r^2 \right) - 3 H^2 \left( 2 m^2 r^2 + k^2 r^4 \right) \right) - 3 i b z D b \phi^5 m r^{1+n z} \left( -12 \right. \right. \right. \\
& \quad \left. \left. H^2 m^2 (-1+n z) r^2 + 9 (-1+2 n z) r^4 + H^4 \left( m^4 (-3+2 n z) - 8 k^2 m^2 r^2 - 3 k^4 r^4 \right) \right) \right. \\
& \quad \left. \left. + 18 b z^4 D b \phi^2 k^2 r^{2+4 n z} \left( -3 r^2 \left( m^2 (7+4 n z) + k^2 (1+2 n z) r^2 \right) + \right. \right. \right. \\
& \quad \left. \left. H^2 \left( 2 m^4 (5+2 n z) + k^2 m^2 (11+8 n z) r^2 + k^4 (3+4 n z) r^4 \right) \right) - \right. \\
& \quad \left. \left. 9 i b z^3 D b \phi^3 m r^{1+3 n z} \left( -3 r^2 \left( m^2 (4+6 n z) + k^2 (1+9 n z) r^2 \right) + \right. \right. \right. \\
& \quad \left. \left. H^2 \left( m^4 (4+6 n z) + k^2 m^2 (-8+11 n z) r^2 + k^4 (2+5 n z) r^4 \right) \right) + 3 b z^2 D b \phi^4 r^{2 n z} \right. \\
& \quad \left. \left( 27 r^4 \left( 2 m^2 + k^2 n z r^2 \right) + 2 H^4 \left( 5 m^6 + k^2 m^4 (7+2 n z) r^2 + 2 k^4 m^2 n z r^4 \right) - \right. \right. \\
& \quad \left. \left. 3 H^2 \left( 16 m^4 r^2 + k^2 m^2 (17+10 n z) r^4 + k^4 (3+2 n z) r^6 \right) \right) \right) \sigma[r] + \\
& \quad 3 m^3 r^3 \left( 12 i b z D b \phi^3 m r^{1+n z} \left( H^2 m^2 - 3 r^2 \right) + 27 i b z^3 D b \phi m r^{1+3 n z} \left( m^2 + k^2 r^2 \right) + \right. \\
& \quad \left. 9 b z^4 k^2 r^{2+4 n z} \left( 2 m^2 + k^2 r^2 \right) + D b \phi^4 \left( -6 H^2 m^2 r^2 + 9 r^4 + H^4 \left( m^4 + 2 k^2 m^2 r^2 \right) \right) \right) + \\
& \quad \left. 3 b z^2 D b \phi^2 r^{2 n z} \left( 3 \left( -4 m^2 r^2 + k^2 r^4 \right) + H^2 \left( 4 m^4 + 6 k^2 m^2 r^2 + 4 k^4 r^4 \right) \right) \right) \sigma[r]^3 \Sigma'[r] + \\
& \quad 3 b z D b \phi r^{n z} \left( 2 D b \phi \left( -i D b \phi^3 m^2 r \left( H^2 m^2 - 3 r^2 \right) \left( -3 r^2 + H^2 \left( m^2 + k^2 r^2 \right) \right) - \right. \right. \\
& \quad \left. \left. 3 b z^3 k^2 m r^{2+3 n z} \left( 2 H^2 \left( m^2 + k^2 r^2 \right)^2 - 3 r^2 \left( 2 m^2 + k^2 r^2 \right) \right) + 3 i b z^2 D b \phi k^2 r^{3+2 n z} \right. \right. \\
& \quad \left. \left. \left( -3 m^2 r^2 + 3 k^2 r^4 + H^2 \left( m^4 + k^2 m^2 r^2 \right) \right) - b z D b \phi^2 m r^{n z} \left( 18 r^4 \left( m^2 - k^2 r^2 \right) + \right. \right. \right. \\
& \quad \left. \left. 2 H^4 \left( m^3 + k^2 m r^2 \right)^2 - 3 H^2 \left( 4 m^4 r^2 + 2 k^2 m^2 r^4 + k^4 r^6 \right) \right) \right) \Omega[r] + r \left( 36 i b z^4 k^4 \right. \\
& \quad \left. m^2 r^{5+4 n z} - 9 b z^3 D b \phi k^2 m r^{2+3 n z} \left( -12 m^2 r^2 + k^2 r^4 + 2 H^2 \left( m^2 + k^2 r^2 \right)^2 \right) - i D b \phi^4 \right. \\
& \quad \left. m^2 r \left( 18 r^4 + H^2 \left( -12 m^2 r^2 + 9 k^2 r^4 \right) + H^4 \left( 2 m^4 - 3 k^2 m^2 r^2 - k^4 r^4 \right) \right) + 3 i b z^2 D b \phi^2 \right. \\
& \quad \left. k^2 r^{3+2 n z} \left( -3 m^2 r^2 + H^2 \left( 13 m^4 + 15 k^2 m^2 r^2 + 2 k^4 r^4 \right) \right) - 3 b z D b \phi^3 m r^{n z} \left( 18 m^2 r^4 - \right. \right. \\
& \quad \left. \left. 6 k^2 r^6 + 2 H^4 \left( m^3 + k^2 m r^2 \right)^2 - H^2 \left( 12 m^4 r^2 + 4 k^2 m^2 r^4 + 3 k^4 r^6 \right) \right) \right) \Omega'[r] \Big) + \\
& \quad b z D b \phi r^{n z} \Sigma[r]^2 \left( 6 b z D b \phi k^2 m r^{5+n z} \left( D b \phi^2 H^2 + 3 b z^2 r^{2 n z} \right) \left( 3 i b z D b \phi k^2 r^{3+n z} + \right. \right. \\
& \quad \left. \left. 3 b z^2 k^2 m r^{2+2 n z} + D b \phi^2 \left( -H^2 m^3 + 3 m r^2 \right) \right) \right) c[r] c'[r] - \\
& \quad 3 r^2 \left( 9 i b z^4 k^4 m r^{4+4 n z} \left( m^2 + k^2 r^2 \right) + 18 b z^3 D b \phi k^4 r^{5+3 n z} \left( 2 m^2 + k^2 r^2 \right) + \right. \\
& \quad \left. 6 b z D b \phi^3 k^2 m^2 r^{3+n z} \left( -9 r^2 + H^2 \left( 3 m^2 + 2 k^2 r^2 \right) \right) + \right. \\
& \quad \left. i D b \phi^4 m^3 \left( 18 r^4 - 3 H^2 \left( 4 m^2 r^2 + 3 k^2 r^4 \right) + H^4 \left( 2 m^4 + 3 k^2 m^2 r^2 + k^4 r^4 \right) \right) + \right. \\
& \quad \left. 3 i b z^2 D b \phi^2 k^2 m r^{2+2 n z} \left( -9 r^2 \left( m^2 + 2 k^2 r^2 \right) + H^2 \left( 3 m^4 + 4 k^2 m^2 r^2 + k^4 r^4 \right) \right) \right) c[r]^4 \Sigma'[r] + \\
& \quad c[r]^2 \left( D b \phi \left( -i D b \phi^5 m^3 r \left( -3 H r^2 + H^3 \left( m^2 + k^2 r^2 \right) \right) \right)^2 - 9 b z^5 k^4 r^{4+5 n z} \right)
\end{aligned}$$

$$\begin{aligned}
& \left( 3 r^2 \left( -m^2 (3 + nz) + k^2 nz r^2 \right) + 2 H^2 \left( m^2 + k^2 r^2 \right) \left( m^2 (3 + 2 nz) + k^2 (1 + 2 nz) r^2 \right) \right) + \\
& 3 bz^3 Db\phi^2 k^2 r^{2+3nz} \left( -18 m^2 (1 + 2 nz) r^4 - 4 H^4 m^2 \left( m^2 + k^2 r^2 \right) \left( m^2 (2 + nz) + \right. \right. \\
& \quad \left. \left. k^2 nz r^2 \right) + 3 H^2 r^2 \left( m^4 (4 + 8 nz) + k^2 m^2 (5 + 2 nz) r^2 + k^4 (1 + 2 nz) r^4 \right) \right) + \\
& 9 i bz^4 Db\phi k^2 m r^{3+4nz} \left( 3 r^2 \left( -m^2 (2 + 3 nz) + k^2 (1 + nz) r^2 \right) + \right. \\
& \quad \left. H^2 \left( m^4 (2 + 3 nz) + 2 k^2 m^2 (-2 + 5 nz) r^2 + k^4 (2 + 7 nz) r^4 \right) \right) + 3 i bz^2 Db\phi^3 m r^{1+2nz} \\
& \left( 9 m^2 (2 + 3 nz) r^4 - 3 H^2 r^2 \left( m^4 (4 + 6 nz) + k^2 m^2 (-3 + 2 nz) r^2 + 2 k^4 (1 + 2 nz) r^4 \right) + \right. \\
& \quad \left. H^4 \left( m^6 (2 + 3 nz) + k^2 m^4 (-15 + 2 nz) r^2 - k^4 m^2 (12 + nz) r^4 - 3 k^6 r^6 \right) \right) - \\
& bz Db\phi^4 H^2 m^2 r^{nz} \left( 2 H^4 \left( m^6 - k^4 m^2 r^4 \right) - 3 H^2 \left( 4 m^4 r^2 + k^2 m^2 (7 + 3 nz) r^4 + k^4 nz r^6 \right) + \right. \\
& \quad \left. 9 \left( 2 m^2 r^4 + k^2 (1 + 3 nz) r^6 \right) \right) + 3 m^2 r^3 \left( 18 i bz^4 k^2 m r^{3+4nz} \left( m^2 + k^2 r^2 \right) + \right. \\
& 6 bz^3 Db\phi k^2 r^{2+3nz} \left( 3 k^2 r^4 + H^2 \left( m^2 + k^2 r^2 \right)^2 \right) + 3 i bz^2 Db\phi^2 m r^{1+2nz} \\
& \left( m^2 + k^2 r^2 \right) \left( -18 r^2 + H^2 \left( 6 m^2 + k^2 r^2 \right) \right) + i Db\phi^4 m r \left( 18 r^4 - 3 H^2 \left( 4 m^2 r^2 + 3 k^2 r^4 \right) + \right. \\
& \quad \left. H^4 \left( 2 m^4 + 3 k^2 m^2 r^2 + k^4 r^4 \right) \right) + bz Db\phi^3 r^{nz} \left( 18 r^4 \left( m^2 - k^2 r^2 \right) + \right. \\
& \quad \left. 2 H^4 \left( m^3 + k^2 m r^2 \right)^2 + H^2 \left( -12 m^4 r^2 + 9 k^2 m^2 r^4 + 9 k^4 r^6 \right) \right) \sigma[r]^2 \Sigma'[r] + \\
& m r^2 \sigma[r] \left( Db\phi m \left( i Db\phi^5 m r \left( -3 H r^2 + H^3 \left( m^2 + k^2 r^2 \right) \right)^2 + 9 bz^5 k^2 r^{2+5nz} \right. \right. \\
& \quad \left. \left( 3 r^2 \left( -m^2 (3 + nz) + k^2 nz r^2 \right) + 2 H^2 \left( m^2 + k^2 r^2 \right) \left( m^2 (3 + 2 nz) + k^2 (1 + 2 nz) r^2 \right) \right) - \right. \\
& \quad \left. 9 i bz^4 Db\phi m r^{1+4nz} \left( -3 r^2 \left( 2 m^2 (1 + nz) + k^2 (-1 + nz) r^2 \right) + \right. \right. \\
& \quad \left. \left. 2 H^2 \left( m^4 (1 + nz) + k^2 m^2 (-2 + nz) r^2 - k^4 r^4 \right) \right) - 3 i bz^2 Db\phi^3 m r^{1+2nz} \right. \\
& \quad \left( 9 (-1 + 3 nz) r^4 + 3 H^2 r^2 \left( m^2 (4 - 6 nz) + 3 k^2 r^2 \right) + H^4 \left( 3 m^4 (-1 + nz) - \right. \right. \\
& \quad \left. \left. 10 k^2 m^2 r^2 - 3 k^4 (1 + nz) r^4 \right) \right) - bz Db\phi^4 H^2 r^{nz} \left( -2 H^4 \left( m^6 - k^4 m^2 r^4 \right) + 3 H^2 \right. \\
& \quad \left. \left( 4 m^4 r^2 + k^2 m^2 (7 + 3 nz) r^4 + k^4 (2 + nz) r^6 \right) - 9 \left( 2 m^2 r^4 + k^2 (1 + 3 nz) r^6 \right) \right) + \\
& 3 bz^3 Db\phi^2 r^{3nz} \left( 27 m^2 r^4 - 9 k^2 nz r^6 + H^4 \left( m^2 + k^2 r^2 \right)^2 \left( 5 m^2 + k^2 (3 + 4 nz) r^2 \right) - \right. \\
& \quad \left. 3 H^2 \left( 8 m^4 r^2 + k^2 m^2 (13 + 4 nz) r^4 + k^4 (3 + 4 nz) r^6 \right) \right) \sigma[r] + \\
& 3 bz m^3 r^{3+nz} \left( -12 i bz Db\phi^2 m r^{1+nz} \left( H^2 m^2 - 3 r^2 \right) - 9 i bz^3 m r^{1+3nz} \left( m^2 + k^2 r^2 \right) - \right. \\
& \quad \left. 6 bz^2 Db\phi m^2 r^{2nz} \left( -3 r^2 + H^2 \left( m^2 + k^2 r^2 \right) \right) - Db\phi^3 H^2 k^2 r^2 \left( 9 r^2 + 2 H^2 \left( m^2 + k^2 r^2 \right) \right) \right) \\
& \sigma[r]^3 \Sigma'[r] - 3 bz Db\phi r^{nz} \left( -2 bz Db\phi^2 r^{nz} \left( -3 m^2 r^2 + H^2 \left( m^2 + k^2 r^2 \right)^2 \right) \right. \\
& \quad \left. \left( i Db\phi \left( H^2 m^2 r - 3 r^3 \right) + bz m r^{nz} \left( -3 r^2 + H^2 \left( m^2 + k^2 r^2 \right) \right) \right) \Omega[r] + \right. \\
& \quad \left. r \left( 18 bz^4 k^2 m^3 r^{4+4nz} - 2 Db\phi^4 H^2 k^2 m r^4 \left( H^2 m^2 - 3 r^2 \right) + 6 i bz^3 Db\phi k^2 m^2 \right. \right. \\
& \quad \left. \left. r^{3+3nz} \left( 3 r^2 + 2 H^2 \left( m^2 + k^2 r^2 \right) \right) - 3 bz^2 Db\phi^2 m r^{2nz} \left( 9 m^2 r^4 + H^4 \left( m^2 + k^2 r^2 \right)^3 + \right. \right. \\
& \quad \left. \left. H^2 \left( -6 m^4 r^2 - 5 k^2 m^2 r^4 + k^4 r^6 \right) \right) + i bz Db\phi^3 r^{1+nz} \left( -18 m^2 r^4 + 3 H^2 \right. \right. \\
& \quad \left. \left. \left( 4 m^4 r^2 - k^2 m^2 r^4 \right) + H^4 \left( -2 m^6 + k^2 m^4 r^2 + 4 k^4 m^2 r^4 + k^6 r^6 \right) \right) \right) \Omega'[r] \right) \right) \right) \Big/ \\
& \left( 6 r \Sigma[r]^2 \left( bz^2 Db\phi^2 r^{2nz} \left( -3 m^2 r^2 + H^2 \left( m^2 + k^2 r^2 \right)^2 \right) - m^2 r^2 \left( 3 bz^2 r^{2nz} \left( m^2 + k^2 r^2 \right) + \right. \right. \right. \\
& \quad \left. \left. Db\phi^2 \left( -3 r^2 + H^2 \left( m^2 + k^2 r^2 \right) \right) \right) \sigma[r]^2 \Sigma[r] + 3 m^4 r^4 \sigma[r]^4 \Sigma[r]^2 + \right. \\
& \quad \left. c[r]^2 \Sigma[r] \left( -6 i bz Db\phi k^2 m r^{3+nz} + 3 bz^2 k^2 r^{2+2nz} \left( m^2 + k^2 r^2 \right) + \right. \right. \\
& \quad \left. \left. Db\phi^2 m^2 \left( -3 r^2 + H^2 \left( m^2 + k^2 r^2 \right) \right) - 3 m^2 r^2 \left( m^2 + k^2 r^2 \right) \sigma[r]^2 \Sigma[r] \right) \right)^2 \Omega[r] \Big)
\end{aligned}$$

$$\begin{aligned}
AO = & \frac{1}{6} \left( -6 m^2 \sigma[r]^2 + \frac{2 Db\phi^2 H^2 m^2}{r^2 \Sigma[r]} - \frac{6 i bz Db\phi m r^{-1+nz}}{\Sigma[r]} + \right. \\
& \frac{6 bz^2 k^2 r^{2nz}}{\Sigma[r]} + \frac{6 bz^2 r^{-2+2nz}}{\Sigma[r]} - \frac{6 bz^2 nz r^{-2+2nz}}{\Sigma[r]} - \frac{12 bz^2 nz^2 r^{-2+2nz}}{\Sigma[r]} - \\
& \left( 6 m^2 r^2 K^2[r] \sigma[r]^2 \Sigma[r] \left( Db\phi^2 \left( -3 r^2 + H^2 \left( m^2 + k^2 r^2 \right) \right) + 3 k^2 r^2 c[r]^2 \Sigma[r] - 3 m^2 r^2 \sigma[r]^2 \Sigma[r] \right) \right) / \\
& \left( bz^2 Db\phi^2 r^{2nz} \left( -3 m^2 r^2 + H^2 \left( m^2 + k^2 r^2 \right)^2 \right) - \right. \\
& \quad m^2 r^2 \left( 3 bz^2 r^{2nz} \left( m^2 + k^2 r^2 \right) + Db\phi^2 \left( -3 r^2 + H^2 \left( m^2 + k^2 r^2 \right) \right) \right) \sigma[r]^2 \Sigma[r] + \\
& \quad \left. 3 m^4 r^4 \sigma[r]^4 \Sigma[r]^2 + c[r]^2 \Sigma[r] \left( -6 i bz Db\phi k^2 m r^{3+nz} + 3 bz^2 k^2 r^{2+2nz} \left( m^2 + k^2 r^2 \right) + \right. \right.
\end{aligned}$$

[illegible]

$$\begin{aligned}
& 9 m^3 r^3 \sigma[r]^2 \Sigma[r]^2 \Omega'[r]) / ((b z^2 D b \phi^2 r^{2 n z} (-3 m^2 r^2 + H^2 (m^2 + k^2 r^2))^2) - \\
& m^2 r^2 (3 b z^2 r^{2 n z} (m^2 + k^2 r^2) + D b \phi^2 (-3 r^2 + H^2 (m^2 + k^2 r^2))) \sigma[r]^2 \Sigma[r] + \\
& 3 m^4 r^4 \sigma[r]^4 \Sigma[r]^2 + c[r]^2 \Sigma[r] (-6 i b z D b \phi k^2 m r^{3+n z} + 3 b z^2 k^2 r^{2+2 n z} (m^2 + k^2 r^2) + \\
& D b \phi^2 m^2 (-3 r^2 + H^2 (m^2 + k^2 r^2)) - 3 m^2 r^2 (m^2 + k^2 r^2) \sigma[r]^2 \Sigma[r])) \Omega[r] + \\
& (4 \Omega[r] (-3 m^3 r^2 \sigma[r]^3 \Sigma[r] (3 m c[r]^2 \Sigma[r]^2 - 3 i b z D b \phi r^{2+n z} \Sigma'[r] + \\
& \Sigma[r] (D b \phi^2 H^2 m + 3 b z^2 m (1+n z) r^{2 n z} + 3 i b z D b \phi n z r^{1+n z} + 3 m r c[r]^2 \Sigma'[r])) + \\
& m \sigma[r] (3 (3 i b z D b \phi k^2 (-1+n z) r^{3+n z} + 3 b z^2 k^2 m r^{2+2 n z} + D b \phi^2 m (-3 r^2 + H^2 (m^2 + 2 k^2 r^2))) \\
& c[r]^2 \Sigma[r]^2 - 3 i b z D b \phi^3 r^{2+n z} (-3 r^2 + H^2 (m^2 + k^2 r^2)) \Sigma'[r] + \\
& D b \phi \Sigma[r] (-9 i b z^3 k^2 n z r^{3+3 n z} + D b \phi^3 H^2 m (-3 r^2 + H^2 (m^2 + k^2 r^2)) + 3 b z^2 D b \phi m \\
& (1+n z) r^{2 n z} (-3 r^2 + H^2 (m^2 + k^2 r^2)) + 3 i b z D b \phi^2 n z r^{1+n z} (-3 r^2 + H^2 (m^2 + k^2 r^2)) + \\
& 3 r (-6 i b z k^2 r^{3+n z} + D b \phi m (-3 r^2 + H^2 (m^2 + k^2 r^2))) c[r]^2 \Sigma'[r])) - \\
& 9 m^2 r^3 \sigma[r]^2 \Sigma[r]^2 (b z^2 r^{2 n z} (m^2 + k^2 r^2) + m^2 c[r]^2 \Sigma[r]) \Omega'[r] + \\
& 3 r \Sigma[r] (b z^2 D b \phi^2 r^{2 n z} (-3 m^2 r^2 + H^2 (m^2 + k^2 r^2))^2) + (-6 i b z D b \phi k^2 m r^{3+n z} + 3 b z^2 k^2 \\
& r^{2+2 n z} (m^2 + k^2 r^2) + D b \phi^2 m^2 (-3 r^2 + H^2 (m^2 + k^2 r^2))) c[r]^2 \Sigma[r] \Omega'[r]) / \\
& (\Sigma[r] (b z^2 D b \phi^2 r^{2 n z} (-3 m^2 r^2 + H^2 (m^2 + k^2 r^2))^2) - m^2 r^2 (3 b z^2 r^{2 n z} (m^2 + k^2 r^2) + \\
& D b \phi^2 (-3 r^2 + H^2 (m^2 + k^2 r^2))) \sigma[r]^2 \Sigma[r] + 3 m^4 r^4 \sigma[r]^4 \Sigma[r]^2 + \\
& c[r]^2 \Sigma[r] (-6 i b z D b \phi k^2 m r^{3+n z} + 3 b z^2 k^2 r^{2+2 n z} (m^2 + k^2 r^2) + \\
& D b \phi^2 m^2 (-3 r^2 + H^2 (m^2 + k^2 r^2)) - 3 m^2 r^2 (m^2 + k^2 r^2) \sigma[r]^2 \Sigma[r])) + \\
& (2 (D b \phi^2 H^2 + 3 b z^2 n z r^{2 n z}) (3 b z D b \phi^2 r^{1+n z} (i D b \phi m r (-3 r^2 + H^2 (m^2 + k^2 r^2)) + \\
& b z r^{n z} (-3 m^2 r^2 + 3 k^2 r^4 + H^2 (m^2 + k^2 r^2))) \Sigma'[r] - \\
& \Sigma[r] (-9 i b z^3 D b \phi k^2 m (1+2 n z) r^{3+3 n z} + 9 b z^4 k^2 n z r^{2+4 n z} (m^2 + k^2 r^2) + D b \phi^4 H^2 m^2 (-3 r^2 + H^2 \\
& (m^2 + k^2 r^2)) + 3 b z^2 D b \phi^2 r^{2 n z} (3 n z r^2 (-m^2 + k^2 r^2) + H^2 (m^2 n z - k^2 r^2) (m^2 + k^2 r^2)) + \\
& 3 i b z D b \phi^3 m r^{1+n z} (-3 n z r^2 + H^2 (m^2 n z + k^2 (-1+n z) r^2)) + 3 m^2 r^3 \\
& (3 i b z D b \phi m r^{1+n z} + 3 b z^2 r^{2 n z} (m^2 + k^2 r^2) + D b \phi^2 (-3 r^2 + H^2 (m^2 + k^2 r^2))) \sigma[r]^2 \Sigma'[r]) + \\
& 9 m^4 r^4 \sigma[r]^3 \Sigma[r]^3 (\sigma[r] + r \Omega'[r]) + 3 m r^2 \sigma[r] \Sigma[r]^2 \\
& (m (D b \phi^2 (3 - H^2 k^2) r^2 + 3 i b z D b \phi m n z r^{1+n z} + 3 b z^2 r^{2 n z} (m^2 n z + k^2 (-1+n z) r^2)) \sigma[r] + \\
& 3 m^3 r^3 \sigma[r]^3 \Sigma'[r] - D b \phi r (-3 i b z k^2 r^{3+n z} + D b \phi m (-3 r^2 + H^2 (m^2 + k^2 r^2))) \Omega'[r])) / \\
& (3 r^2 \Sigma[r]^2 (b z^2 D b \phi^2 r^{2 n z} (-3 m^2 r^2 + H^2 (m^2 + k^2 r^2))^2) - m^2 r^2 \\
& (3 b z^2 r^{2 n z} (m^2 + k^2 r^2) + D b \phi^2 (-3 r^2 + H^2 (m^2 + k^2 r^2))) \sigma[r]^2 \Sigma[r] + \\
& 3 m^4 r^4 \sigma[r]^4 \Sigma[r]^2 + c[r]^2 \Sigma[r] (-6 i b z D b \phi k^2 m r^{3+n z} + 3 b z^2 k^2 r^{2+2 n z} (m^2 + k^2 r^2) + \\
& D b \phi^2 m^2 (-3 r^2 + H^2 (m^2 + k^2 r^2)) - 3 m^2 r^2 (m^2 + k^2 r^2) \sigma[r]^2 \Sigma[r])) - \\
& (2 c[r]^2 (-3 b z D b \phi^2 r^{1+n z} (i D b \phi m r (-3 r^2 + H^2 (m^2 + k^2 r^2)) + b z r^{n z} \\
& (-3 m^2 r^2 + 3 k^2 r^4 + H^2 (m^2 + k^2 r^2))) \Sigma'[r] + \Sigma[r] (-9 i b z^3 D b \phi k^2 m (1+2 n z) r^{3+3 n z} + \\
& 9 b z^4 k^2 n z r^{2+4 n z} (m^2 + k^2 r^2) + D b \phi^4 H^2 m^2 (-3 r^2 + H^2 (m^2 + k^2 r^2)) + \\
& 3 b z^2 D b \phi^2 r^{2 n z} (3 n z r^2 (-m^2 + k^2 r^2) + H^2 (m^2 n z - k^2 r^2) (m^2 + k^2 r^2)) + \\
& 3 i b z D b \phi^3 m r^{1+n z} (-3 n z r^2 + H^2 (m^2 n z + k^2 (-1+n z) r^2)) + 3 m^2 r^3 \\
& (3 i b z D b \phi m r^{1+n z} + 3 b z^2 r^{2 n z} (m^2 + k^2 r^2) + D b \phi^2 (-3 r^2 + H^2 (m^2 + k^2 r^2))) \sigma[r]^2 \Sigma'[r]) - \\
& 9 m^4 r^4 \sigma[r]^3 \Sigma[r]^3 (\sigma[r] + r \Omega'[r]) + 3 m r^2 \sigma[r] \Sigma[r]^2 \\
& (m (D b \phi^2 (-3 + H^2 k^2) r^2 - 3 i b z D b \phi m n z r^{1+n z} - 3 b z^2 r^{2 n z} (m^2 n z + k^2 (-1+n z) r^2)) \sigma[r] - \\
& 3 m^3 r^3 \sigma[r]^3 \Sigma'[r] + D b \phi r (-3 i b z k^2 r^{3+n z} + D b \phi m (-3 r^2 + H^2 (m^2 + k^2 r^2))) \Omega'[r])) / \\
& (r^2 \Sigma[r] (b z^2 D b \phi^2 r^{2 n z} (-3 m^2 r^2 + H^2 (m^2 + k^2 r^2))^2) - m^2 r^2 (3 b z^2 r^{2 n z} (m^2 + k^2 r^2) + \\
& D b \phi^2 (-3 r^2 + H^2 (m^2 + k^2 r^2))) \sigma[r]^2 \Sigma[r] + 3 m^4 r^4 \sigma[r]^4 \Sigma[r]^2 + \\
& c[r]^2 \Sigma[r] (-6 i b z D b \phi k^2 m r^{3+n z} + 3 b z^2 k^2 r^{2+2 n z} (m^2 + k^2 r^2) + \\
& D b \phi^2 m^2 (-3 r^2 + H^2 (m^2 + k^2 r^2)) - 3 m^2 r^2 (m^2 + k^2 r^2) \sigma[r]^2 \Sigma[r])) + \\
& (4 c[r] c'[r] (-3 b z D b \phi^2 r^{1+n z} (i D b \phi m r (-3 r^2 + H^2 (m^2 + k^2 r^2)) + b z r^{n z} \\
& (-3 m^2 r^2 + 3 k^2 r^4 + H^2 (m^2 + k^2 r^2))) \Sigma'[r] + \Sigma[r] (-9 i b z^3 D b \phi k^2 m (1+2 n z) r^{3+3 n z} +
\end{aligned}$$

[illegible]



$$\begin{aligned}
& (3 m c[r]^2 K^2[r] \sigma[r] \Sigma[r] (D b \phi (-3 i b z k^2 r^{3+n z} + D b \phi m (-3 r^2 + H^2 (m^2 + k^2 r^2))) - \\
& \quad 3 m^3 r^2 \sigma[r]^2 \Sigma[r]) \\
& (2 b z^2 D b \phi^2 r^{2 n z} (-3 m^2 (1 + n z) r^2 + H^2 (m^2 + k^2 r^2) (m^2 n z + k^2 (2 + n z) r^2)) + 2 r c[r] \\
& \quad \Sigma[r] (-6 i b z D b \phi k^2 m r^{3+n z} + 3 b z^2 k^2 r^{2+2 n z} (m^2 + k^2 r^2) + D b \phi^2 m^2 (-3 r^2 + H^2 (m^2 + k^2 r^2))) - \\
& \quad 3 m^2 r^2 (m^2 + k^2 r^2) \sigma[r]^2 \Sigma[r]) c'[r] + 6 m^4 r^4 \sigma[r]^4 \Sigma[r] (2 \Sigma[r] + r \Sigma'[r]) - \\
& \quad m^2 r^2 \sigma[r]^2 (2 (3 b z^2 r^{2 n z} (m^2 (1 + n z) + k^2 (2 + n z) r^2) + D b \phi^2 (-6 r^2 + H^2 (m^2 + 2 k^2 r^2))) \\
& \quad \Sigma[r] + r (3 b z^2 r^{2 n z} (m^2 + k^2 r^2) + D b \phi^2 (-3 r^2 + H^2 (m^2 + k^2 r^2))) \Sigma'[r]) - \\
& \quad 2 m^2 r^3 (3 b z^2 r^{2 n z} (m^2 + k^2 r^2) + D b \phi^2 (-3 r^2 + H^2 (m^2 + k^2 r^2))) \sigma[r] \Sigma[r] \Omega'[r] + \\
& \quad 12 m^4 r^5 \sigma[r]^3 \Sigma[r]^2 \Omega'[r] + r c[r]^2 \\
& \quad ((-6 i b z D b \phi k^2 m r^{3+n z} + 3 b z^2 k^2 r^{2+2 n z} (m^2 + k^2 r^2) + D b \phi^2 m^2 (-3 r^2 + H^2 (m^2 + k^2 r^2))) \\
& \quad \Sigma'[r] + 2 r \Sigma[r] (D b \phi^2 (-3 + H^2 k^2) m^2 - 3 i b z D b \phi k^2 m (3 + n z) r^{1+n z} + 3 b z^2 \\
& \quad k^2 r^{2 n z} (m^2 (1 + n z) + k^2 (2 + n z) r^2) - 3 m^2 r (m^2 + k^2 r^2) \sigma[r]^2 \Sigma'[r]) - \\
& \quad 6 m^2 r \sigma[r] \Sigma[r]^2 ((m^2 + 2 k^2 r^2) \sigma[r] + r (m^2 + k^2 r^2) \Omega'[r]))) / \\
& ((b z^2 D b \phi^2 r^{2 n z} (-3 m^2 r^2 + H^2 (m^2 + k^2 r^2)^2) - m^2 r^2 (3 b z^2 r^{2 n z} (m^2 + k^2 r^2) + \\
& \quad D b \phi^2 (-3 r^2 + H^2 (m^2 + k^2 r^2))) \sigma[r]^2 \Sigma[r] + 3 m^4 r^4 \sigma[r]^4 \Sigma[r]^2 + \\
& \quad c[r]^2 \Sigma[r] (-6 i b z D b \phi k^2 m r^{3+n z} + 3 b z^2 k^2 r^{2+2 n z} (m^2 + k^2 r^2) + \\
& \quad D b \phi^2 m^2 (-3 r^2 + H^2 (m^2 + k^2 r^2)) - 3 m^2 r^2 (m^2 + k^2 r^2) \sigma[r]^2 \Sigma[r]))^2 \Omega[r]) - \\
& (2 c[r]^2 (-3 b z D b \phi^2 r^{1+n z} (i D b \phi m r (-3 r^2 + H^2 (m^2 + k^2 r^2)) + b z r^{n z} \\
& \quad (-3 m^2 r^2 + 3 k^2 r^4 + H^2 (m^2 + k^2 r^2)^2)) \Sigma'[r] + \Sigma[r] (-9 i b z^3 D b \phi k^2 m (1 + 2 n z) r^{3+3 n z} + \\
& \quad 9 b z^4 k^2 n z r^{2+4 n z} (m^2 + k^2 r^2) + D b \phi^4 H^2 m^2 (-3 r^2 + H^2 (m^2 + k^2 r^2)) + \\
& \quad 3 b z^2 D b \phi^2 r^{2 n z} (3 n z r^2 (-m^2 + k^2 r^2) + H^2 (m^2 n z - k^2 r^2) (m^2 + k^2 r^2)) + \\
& \quad 3 i b z D b \phi^3 m r^{1+n z} (-3 n z r^2 + H^2 (m^2 n z + k^2 (-1 + n z) r^2)) + 3 m^2 r^3 \\
& \quad (3 i b z D b \phi m r^{1+n z} + 3 b z^2 r^{2 n z} (m^2 + k^2 r^2) + D b \phi^2 (-3 r^2 + H^2 (m^2 + k^2 r^2))) \sigma[r]^2 \Sigma'[r]) - \\
& \quad 9 m^4 r^4 \sigma[r]^3 \Sigma[r]^3 (\sigma[r] + r \Omega'[r]) + 3 m r^2 \sigma[r] \Sigma[r]^2 \\
& \quad (m (D b \phi^2 (-3 + H^2 k^2) r^2 - 3 i b z D b \phi m n z r^{1+n z} - 3 b z^2 r^{2 n z} (m^2 n z + k^2 (-1 + n z) r^2)) \sigma[r] - \\
& \quad 3 m^3 r^3 \sigma[r]^3 \Sigma'[r] + D b \phi r (-3 i b z k^2 r^{3+n z} + D b \phi m (-3 r^2 + H^2 (m^2 + k^2 r^2))) \Omega'[r])) \\
& (2 b z^2 D b \phi^2 r^{2 n z} (-3 m^2 (1 + n z) r^2 + H^2 (m^2 + k^2 r^2) (m^2 n z + k^2 (2 + n z) r^2)) + 2 r c[r] \\
& \quad \Sigma[r] (-6 i b z D b \phi k^2 m r^{3+n z} + 3 b z^2 k^2 r^{2+2 n z} (m^2 + k^2 r^2) + D b \phi^2 m^2 (-3 r^2 + H^2 (m^2 + k^2 r^2))) - \\
& \quad 3 m^2 r^2 (m^2 + k^2 r^2) \sigma[r]^2 \Sigma[r]) c'[r] + 6 m^4 r^4 \sigma[r]^4 \Sigma[r] (2 \Sigma[r] + r \Sigma'[r]) - \\
& \quad m^2 r^2 \sigma[r]^2 (2 (3 b z^2 r^{2 n z} (m^2 (1 + n z) + k^2 (2 + n z) r^2) + D b \phi^2 (-6 r^2 + H^2 (m^2 + 2 k^2 r^2))) \\
& \quad \Sigma[r] + r (3 b z^2 r^{2 n z} (m^2 + k^2 r^2) + D b \phi^2 (-3 r^2 + H^2 (m^2 + k^2 r^2))) \Sigma'[r]) - \\
& \quad 2 m^2 r^3 (3 b z^2 r^{2 n z} (m^2 + k^2 r^2) + D b \phi^2 (-3 r^2 + H^2 (m^2 + k^2 r^2))) \sigma[r] \Sigma[r] \Omega'[r] + \\
& \quad 12 m^4 r^5 \sigma[r]^3 \Sigma[r]^2 \Omega'[r] + r c[r]^2 \\
& \quad ((-6 i b z D b \phi k^2 m r^{3+n z} + 3 b z^2 k^2 r^{2+2 n z} (m^2 + k^2 r^2) + D b \phi^2 m^2 (-3 r^2 + H^2 (m^2 + k^2 r^2))) \\
& \quad \Sigma'[r] + 2 r \Sigma[r] (D b \phi^2 (-3 + H^2 k^2) m^2 - 3 i b z D b \phi k^2 m (3 + n z) r^{1+n z} + 3 b z^2 \\
& \quad k^2 r^{2 n z} (m^2 (1 + n z) + k^2 (2 + n z) r^2) - 3 m^2 r (m^2 + k^2 r^2) \sigma[r]^2 \Sigma'[r]) - \\
& \quad 6 m^2 r \sigma[r] \Sigma[r]^2 ((m^2 + 2 k^2 r^2) \sigma[r] + r (m^2 + k^2 r^2) \Omega'[r]))) / \\
& (r^2 \Sigma[r] (b z^2 D b \phi^2 r^{2 n z} (-3 m^2 r^2 + H^2 (m^2 + k^2 r^2)^2) - m^2 r^2 (3 b z^2 r^{2 n z} (m^2 + k^2 r^2) + \\
& \quad D b \phi^2 (-3 r^2 + H^2 (m^2 + k^2 r^2))) \sigma[r]^2 \Sigma[r] + 3 m^4 r^4 \sigma[r]^4 \Sigma[r]^2 + \\
& \quad c[r]^2 \Sigma[r] (-6 i b z D b \phi k^2 m r^{3+n z} + 3 b z^2 k^2 r^{2+2 n z} (m^2 + k^2 r^2) + \\
& \quad D b \phi^2 m^2 (-3 r^2 + H^2 (m^2 + k^2 r^2)) - 3 m^2 r^2 (m^2 + k^2 r^2) \sigma[r]^2 \Sigma[r]))^2) - \\
& (2 b z^2 m r^{-2+2 n z} (-3 i b z D b \phi^3 r^{2+n z} (-3 r^2 + H^2 (m^2 + k^2 r^2)) \Sigma'[r] + D b \phi \Sigma[r] \\
& \quad (D b \phi^3 H^4 m^3 - 3 D b \phi^3 H^2 m r^2 + D b \phi^3 H^4 k^2 m r^2 + 3 b z^2 D b \phi H^2 m^3 r^{2 n z} + 3 b z^2 D b \phi H^2 m^3 n z r^{2 n z} + \\
& \quad 3 i b z D b \phi^2 H^2 m^2 n z r^{1+n z} - 9 i b z D b \phi^2 n z r^{3+n z} + 3 i b z D b \phi^2 H^2 k^2 n z r^{3+n z} - \\
& \quad 9 b z^2 D b \phi m r^{2+2 n z} + 3 b z^2 D b \phi H^2 k^2 m r^{2+2 n z} - 9 b z^2 D b \phi m n z r^{2+2 n z} +
\end{aligned}$$

$$\begin{aligned}
& 3 \text{bz}^2 \text{Db}\phi \text{H}^2 \text{k}^2 \text{m nz r}^{2+2 \text{nz}} - 9 \text{i bz}^3 \text{k}^2 \text{nz r}^{3+3 \text{nz}} + 3 \text{r} (-6 \text{i bz k}^2 \text{r}^{3+\text{nz}} + \text{Db}\phi \\
& \text{m} (-3 \text{r}^2 + \text{H}^2 (\text{m}^2 + \text{k}^2 \text{r}^2))) \text{c[r]}^2 \Sigma'[\text{r}] + 9 \text{i bz m}^2 \text{r}^{4+\text{nz}} \sigma[\text{r}]^2 \Sigma'[\text{r}] - \\
& 9 \text{m r}^2 \sigma[\text{r}] \Sigma[\text{r}]^3 (\text{m}^2 \text{r}^3 \sigma[\text{r}]^2 \Omega'[\text{r}] + \text{c[r]}^2 (\text{m}^2 \sigma[\text{r}] - \text{k}^2 \text{r}^3 \Omega'[\text{r}])) + 3 \Sigma[\text{r}]^2 \\
& (\text{c[r]}^2 (3 \text{i bz Db}\phi \text{k}^2 (-1 + \text{nz}) \text{r}^{3+\text{nz}} + 3 \text{bz}^2 \text{k}^2 \text{m r}^{2+2 \text{nz}} + \text{Db}\phi^2 \text{m} (-3 \text{r}^2 + \text{H}^2 (\text{m}^2 + 2 \text{k}^2 \text{r}^2)) - 3 \\
& \text{m}^3 \text{r}^3 \sigma[\text{r}]^2 \Sigma'[\text{r}]) + \text{m r}^2 \sigma[\text{r}] (-\text{m} (\text{Db}\phi^2 \text{H}^2 \text{m} + 3 \text{bz}^2 \text{m} (1 + \text{nz}) \text{r}^{2 \text{nz}} + \\
& 3 \text{i bz Db}\phi \text{nz r}^{1+\text{nz}}) \sigma[\text{r}] + \text{Db}\phi^2 \text{r} (-3 \text{r}^2 + \text{H}^2 (\text{m}^2 + \text{k}^2 \text{r}^2)) \Omega'[\text{r}])))) / \\
& (\Sigma[\text{r}]^2 (\text{bz}^2 \text{Db}\phi^2 \text{r}^{2 \text{nz}} (-3 \text{m}^2 \text{r}^2 + \text{H}^2 (\text{m}^2 + \text{k}^2 \text{r}^2)^2) - \text{m}^2 \text{r}^2 (3 \text{bz}^2 \text{r}^{2 \text{nz}} (\text{m}^2 + \text{k}^2 \text{r}^2) + \\
& \text{Db}\phi^2 (-3 \text{r}^2 + \text{H}^2 (\text{m}^2 + \text{k}^2 \text{r}^2))) \sigma[\text{r}]^2 \Sigma[\text{r}] + 3 \text{m}^4 \text{r}^4 \sigma[\text{r}]^4 \Sigma[\text{r}]^2 + \\
& \text{c[r]}^2 \Sigma[\text{r}] (-6 \text{i bz Db}\phi \text{k}^2 \text{m r}^{3+\text{nz}} + 3 \text{bz}^2 \text{k}^2 \text{r}^{2+2 \text{nz}} (\text{m}^2 + \text{k}^2 \text{r}^2) + \\
& \text{Db}\phi^2 \text{m}^2 (-3 \text{r}^2 + \text{H}^2 (\text{m}^2 + \text{k}^2 \text{r}^2)) - 3 \text{m}^2 \text{r}^2 (\text{m}^2 + \text{k}^2 \text{r}^2) \sigma[\text{r}]^2 \Sigma[\text{r}])) + \\
& (4 \text{bz}^2 \text{m nz r}^{-2+2 \text{nz}} (-3 \text{i bz Db}\phi^3 \text{r}^{2+\text{nz}} (-3 \text{r}^2 + \text{H}^2 (\text{m}^2 + \text{k}^2 \text{r}^2)) \Sigma'[\text{r}] + \\
& \text{Db}\phi \Sigma[\text{r}] (\text{Db}\phi^3 \text{H}^4 \text{m}^3 - 3 \text{Db}\phi^3 \text{H}^2 \text{m r}^2 + \text{Db}\phi^3 \text{H}^4 \text{k}^2 \text{m r}^2 + 3 \text{bz}^2 \text{Db}\phi \text{H}^2 \text{m}^3 \text{r}^{2 \text{nz}} + \\
& 3 \text{bz}^2 \text{Db}\phi \text{H}^2 \text{m}^3 \text{nz r}^{2 \text{nz}} + 3 \text{i bz Db}\phi^2 \text{H}^2 \text{m}^2 \text{nz r}^{1+\text{nz}} - 9 \text{i bz Db}\phi^2 \text{nz r}^{3+\text{nz}} + \\
& 3 \text{i bz Db}\phi^2 \text{H}^2 \text{k}^2 \text{nz r}^{3+\text{nz}} - 9 \text{bz}^2 \text{Db}\phi \text{m r}^{2+2 \text{nz}} + 3 \text{bz}^2 \text{Db}\phi \text{H}^2 \text{k}^2 \text{m r}^{2+2 \text{nz}} - \\
& 9 \text{bz}^2 \text{Db}\phi \text{m nz r}^{2+2 \text{nz}} + 3 \text{bz}^2 \text{Db}\phi \text{H}^2 \text{k}^2 \text{m nz r}^{2+2 \text{nz}} - 9 \text{i bz}^3 \text{k}^2 \text{nz r}^{3+3 \text{nz}} + 3 \text{r} (-6 \text{i bz k}^2 \\
& \text{r}^{3+\text{nz}} + \text{Db}\phi \text{m} (-3 \text{r}^2 + \text{H}^2 (\text{m}^2 + \text{k}^2 \text{r}^2))) \text{c[r]}^2 \Sigma'[\text{r}] + 9 \text{i bz m}^2 \text{r}^{4+\text{nz}} \sigma[\text{r}]^2 \Sigma'[\text{r}]) - \\
& 9 \text{m r}^2 \sigma[\text{r}] \Sigma[\text{r}]^3 (\text{m}^2 \text{r}^3 \sigma[\text{r}]^2 \Omega'[\text{r}] + \text{c[r]}^2 (\text{m}^2 \sigma[\text{r}] - \text{k}^2 \text{r}^3 \Omega'[\text{r}])) + 3 \Sigma[\text{r}]^2 \\
& (\text{c[r]}^2 (3 \text{i bz Db}\phi \text{k}^2 (-1 + \text{nz}) \text{r}^{3+\text{nz}} + 3 \text{bz}^2 \text{k}^2 \text{m r}^{2+2 \text{nz}} + \text{Db}\phi^2 \text{m} (-3 \text{r}^2 + \text{H}^2 (\text{m}^2 + 2 \text{k}^2 \text{r}^2)) - 3 \\
& \text{m}^3 \text{r}^3 \sigma[\text{r}]^2 \Sigma'[\text{r}]) + \text{m r}^2 \sigma[\text{r}] (-\text{m} (\text{Db}\phi^2 \text{H}^2 \text{m} + 3 \text{bz}^2 \text{m} (1 + \text{nz}) \text{r}^{2 \text{nz}} + \\
& 3 \text{i bz Db}\phi \text{nz r}^{1+\text{nz}}) \sigma[\text{r}] + \text{Db}\phi^2 \text{r} (-3 \text{r}^2 + \text{H}^2 (\text{m}^2 + \text{k}^2 \text{r}^2)) \Omega'[\text{r}])))) / \\
& (\Sigma[\text{r}]^2 (\text{bz}^2 \text{Db}\phi^2 \text{r}^{2 \text{nz}} (-3 \text{m}^2 \text{r}^2 + \text{H}^2 (\text{m}^2 + \text{k}^2 \text{r}^2)^2) - \text{m}^2 \text{r}^2 (3 \text{bz}^2 \text{r}^{2 \text{nz}} (\text{m}^2 + \text{k}^2 \text{r}^2) + \\
& \text{Db}\phi^2 (-3 \text{r}^2 + \text{H}^2 (\text{m}^2 + \text{k}^2 \text{r}^2))) \sigma[\text{r}]^2 \Sigma[\text{r}] + 3 \text{m}^4 \text{r}^4 \sigma[\text{r}]^4 \Sigma[\text{r}]^2 + \\
& \text{c[r]}^2 \Sigma[\text{r}] (-6 \text{i bz Db}\phi \text{k}^2 \text{m r}^{3+\text{nz}} + 3 \text{bz}^2 \text{k}^2 \text{r}^{2+2 \text{nz}} (\text{m}^2 + \text{k}^2 \text{r}^2) + \\
& \text{Db}\phi^2 \text{m}^2 (-3 \text{r}^2 + \text{H}^2 (\text{m}^2 + \text{k}^2 \text{r}^2)) - 3 \text{m}^2 \text{r}^2 (\text{m}^2 + \text{k}^2 \text{r}^2) \sigma[\text{r}]^2 \Sigma[\text{r}])) - \\
& (\text{c[r]}^2 (-2 \text{r} (-3 \text{bz Db}\phi^2 \text{r}^{1+\text{nz}} (\text{i Db}\phi \text{m r} (-3 \text{r}^2 + \text{H}^2 (\text{m}^2 + \text{k}^2 \text{r}^2)) + \text{bz r}^{\text{nz}} \\
& (-3 \text{m}^2 \text{r}^2 + 3 \text{k}^2 \text{r}^4 + \text{H}^2 (\text{m}^2 + \text{k}^2 \text{r}^2)^2)) \Sigma'[\text{r}] \Omega'[\text{r}] + \\
& \Omega[\text{r}] ((-9 \text{i bz}^3 \text{Db}\phi \text{k}^2 \text{m} (1 + 2 \text{nz}) \text{r}^{3+3 \text{nz}} + 9 \text{bz}^4 \text{k}^2 \text{nz r}^{2+4 \text{nz}} (\text{m}^2 + \text{k}^2 \text{r}^2) + \text{Db}\phi^4 \text{H}^2 \text{m}^2 \\
& (-3 \text{r}^2 + \text{H}^2 (\text{m}^2 + \text{k}^2 \text{r}^2)) - 3 \text{i bz Db}\phi^3 \text{m r}^{1+\text{nz}} (-12 \text{r}^2 + \text{H}^2 (2 \text{m}^2 + 5 \text{k}^2 \text{r}^2)) - 3 \text{bz}^2 \\
& \text{Db}\phi^2 \text{r}^{2 \text{nz}} (\text{H}^2 (\text{m}^2 + \text{k}^2 \text{r}^2) (\text{m}^2 (1 + \text{nz}) + 2 \text{k}^2 (3 + \text{nz}) \text{r}^2) + 3 \text{r}^2 (-\text{m}^2 (3 + \text{nz}) + \text{k}^2 \\
& (5 + \text{nz}) \text{r}^2))) \Sigma'[\text{r}] + 3 \text{m}^2 \text{r}^3 (3 \text{i bz Db}\phi \text{m r}^{1+\text{nz}} + 3 \text{bz}^2 \text{r}^{2 \text{nz}} (\text{m}^2 + \text{k}^2 \text{r}^2) + \\
& \text{Db}\phi^2 (-3 \text{r}^2 + \text{H}^2 (\text{m}^2 + \text{k}^2 \text{r}^2))) \sigma[\text{r}]^2 \Sigma'[\text{r}]^2 - 3 \text{bz Db}\phi^2 \text{r}^{1+\text{nz}} (\text{i Db}\phi \text{m r} \\
& (-3 \text{r}^2 + \text{H}^2 (\text{m}^2 + \text{k}^2 \text{r}^2)) + \text{bz r}^{\text{nz}} (-3 \text{m}^2 \text{r}^2 + 3 \text{k}^2 \text{r}^4 + \text{H}^2 (\text{m}^2 + \text{k}^2 \text{r}^2)^2)) \Sigma''[\text{r}])) - \\
& 2 \Sigma[\text{r}] (\text{r} (-9 \text{i bz}^3 \text{Db}\phi \text{k}^2 \text{m} (1 + 2 \text{nz}) \text{r}^{3+3 \text{nz}} + 9 \text{bz}^4 \text{k}^2 \text{nz r}^{2+4 \text{nz}} (\text{m}^2 + \text{k}^2 \text{r}^2) + \text{Db}\phi^4 \text{H}^2 \\
& \text{m}^2 (-3 \text{r}^2 + \text{H}^2 (\text{m}^2 + \text{k}^2 \text{r}^2)) + 3 \text{bz}^2 \text{Db}\phi^2 \text{r}^{2 \text{nz}} (3 \text{nz r}^2 (-\text{m}^2 + \text{k}^2 \text{r}^2) + \text{H}^2 (\text{m}^2 \text{nz} - \text{k}^2 \text{r}^2) \\
& (\text{m}^2 + \text{k}^2 \text{r}^2)) + 3 \text{i bz Db}\phi^3 \text{m r}^{1+\text{nz}} (-3 \text{nz r}^2 + \text{H}^2 (\text{m}^2 \text{nz} + \text{k}^2 (-1 + \text{nz}) \text{r}^2)) + 3 \text{m}^2 \\
& \text{r}^3 (3 \text{i bz Db}\phi \text{m r}^{1+\text{nz}} + 3 \text{bz}^2 \text{r}^{2 \text{nz}} (\text{m}^2 + \text{k}^2 \text{r}^2) + \text{Db}\phi^2 (-3 \text{r}^2 + \text{H}^2 (\text{m}^2 + \text{k}^2 \text{r}^2))) \\
& \sigma[\text{r}]^2 \Sigma'[\text{r}]) \Omega'[\text{r}] + \Omega[\text{r}] (2 \text{Db}\phi^4 \text{H}^2 (-3 + \text{H}^2 \text{k}^2) \text{m}^2 \text{r}^2 - 27 \text{i bz}^3 \text{Db}\phi \text{k}^2 \text{m} \\
& (1 + 3 \text{nz} + 2 \text{nz}^2) \text{r}^{3+3 \text{nz}} + 18 \text{bz}^4 \text{k}^2 \text{nz r}^{2+4 \text{nz}} (\text{m}^2 (1 + 2 \text{nz}) + 2 \text{k}^2 (1 + \text{nz}) \text{r}^2) + 3 \text{i bz} \\
& \text{Db}\phi^3 \text{m r}^{1+\text{nz}} (-3 \text{nz} (3 + \text{nz}) \text{r}^2 + \text{H}^2 (\text{m}^2 \text{nz} (1 + \text{nz}) + \text{k}^2 (-3 + 2 \text{nz} + \text{nz}^2) \text{r}^2)) + 6 \text{bz}^2 \\
& \text{Db}\phi^2 \text{r}^{2 \text{nz}} (3 \text{nz r}^2 (-\text{m}^2 (1 + \text{nz}) + \text{k}^2 (2 + \text{nz}) \text{r}^2) + \text{H}^2 (\text{m}^4 \text{nz}^2 + \text{k}^2 \text{m}^2 (-1 + \text{nz}^2) \text{r}^2 - \\
& \text{k}^4 (2 + \text{nz}) \text{r}^4)) - 18 \text{m}^4 \text{r}^6 \sigma[\text{r}]^4 \Sigma'[\text{r}]^2 + 6 \text{m r}^4 (3 \text{i bz Db}\phi \text{r}^{1+\text{nz}} (\text{m}^2 - \text{k}^2 \text{r}^2) + \\
& 3 \text{bz}^2 \text{m r}^{2 \text{nz}} (\text{m}^2 + \text{k}^2 \text{r}^2) + 2 \text{Db}\phi^2 \text{m} (-3 \text{r}^2 + \text{H}^2 (\text{m}^2 + \text{k}^2 \text{r}^2))) \sigma[\text{r}] \Sigma'[\text{r}] \\
& \Omega'[\text{r}] + 3 \text{m}^2 \text{r}^3 \sigma[\text{r}]^2 ((-3 \text{i bz Db}\phi \text{m} (-4 + \text{nz}) \text{r}^{1+\text{nz}} + 3 \text{bz}^2 \text{r}^{2 \text{nz}} (3 \text{m}^2 + 7 \text{k}^2 \text{r}^2) + \\
& \text{Db}\phi^2 (-21 \text{r}^2 + \text{H}^2 (3 \text{m}^2 + 7 \text{k}^2 \text{r}^2))) \Sigma'[\text{r}] + \text{r} (3 \text{i bz Db}\phi \text{m r}^{1+\text{nz}} + \\
& 3 \text{bz}^2 \text{r}^{2 \text{nz}} (\text{m}^2 + \text{k}^2 \text{r}^2) + \text{Db}\phi^2 (-3 \text{r}^2 + \text{H}^2 (\text{m}^2 + \text{k}^2 \text{r}^2))) \Sigma''[\text{r}])) + \\
& 9 \text{m}^4 \text{r}^4 \sigma[\text{r}]^2 \Sigma[\text{r}]^3 (6 \text{r}^2 \Omega[\text{r}] \Omega'[\text{r}]^2 + 2 \sigma[\text{r}]^2 (4 \Omega[\text{r}] + \text{r} \Omega'[\text{r}]) + \text{r} \sigma[\text{r}])
\end{aligned}$$

[illegible]

$$\begin{aligned}
& \left( \text{Db}\phi^2 m^2 (-3 r^2 + H^2 (m^2 + k^2 r^2)) - 3 m^2 r^2 (m^2 + k^2 r^2) \sigma[r]^2 \Sigma[r] \right) \Omega[r] + \\
& \left( 3 \text{Db}\phi^2 H^2 k^2 m r^4 K^2[r] \sigma[r] \Sigma[r] (\text{bz} \text{Db}\phi (1 + nz) r^{nz} + 2 m c[r] \Sigma[r] c'[r] + m c[r]^2 \Sigma'[r]) \right) / \\
& \left( (\text{bz}^2 \text{Db}\phi^2 r^{2nz} (-3 m^2 r^2 + H^2 (m^2 + k^2 r^2))^2 - \right. \\
& \quad m^2 r^2 (3 \text{bz}^2 r^{2nz} (m^2 + k^2 r^2) + \text{Db}\phi^2 (-3 r^2 + H^2 (m^2 + k^2 r^2))) \sigma[r]^2 \Sigma[r] + \\
& \quad 3 m^4 r^4 \sigma[r]^4 \Sigma[r]^2 + c[r]^2 \Sigma[r] (-6 \text{bz} \text{Db}\phi k^2 m r^{3+nz} + 3 \text{bz}^2 k^2 r^{2+2nz} (m^2 + k^2 r^2) + \\
& \quad \text{Db}\phi^2 m^2 (-3 r^2 + H^2 (m^2 + k^2 r^2)) - 3 m^2 r^2 (m^2 + k^2 r^2) \sigma[r]^2 \Sigma[r]) \Omega[r] - \\
& \quad \left. \frac{6 \text{bz}^2 r^{2nz} \Omega'[r]}{\sigma[r]} - (3 \text{Db}\phi^2 H^2 k^2 m r^4 K^2[r] \sigma[r] \Sigma[r] (\text{bz} \text{Db}\phi r^{1+nz} + m c[r]^2 \Sigma[r]) \Omega'[r]) \right) / \\
& \left( (\text{bz}^2 \text{Db}\phi^2 r^{2nz} (-3 m^2 r^2 + H^2 (m^2 + k^2 r^2))^2 - \right. \\
& \quad m^2 r^2 (3 \text{bz}^2 r^{2nz} (m^2 + k^2 r^2) + \text{Db}\phi^2 (-3 r^2 + H^2 (m^2 + k^2 r^2))) \sigma[r]^2 \Sigma[r] + \\
& \quad 3 m^4 r^4 \sigma[r]^4 \Sigma[r]^2 + c[r]^2 \Sigma[r] (-6 \text{bz} \text{Db}\phi k^2 m r^{3+nz} + 3 \text{bz}^2 k^2 r^{2+2nz} (m^2 + k^2 r^2) + \\
& \quad \text{Db}\phi^2 m^2 (-3 r^2 + H^2 (m^2 + k^2 r^2)) - 3 m^2 r^2 (m^2 + k^2 r^2) \sigma[r]^2 \Sigma[r]) \Omega[r]^2 + \\
& \quad \left. (3 \text{bz}^2 m^2 r^{2+2nz} K^2[r] \sigma[r] \Sigma[r] (\text{Db}\phi^2 (-3 r^2 + H^2 (m^2 + k^2 r^2)) + 3 k^2 r^2 c[r]^2 \Sigma[r] - \right. \\
& \quad \left. 3 m^2 r^2 \sigma[r]^2 \Sigma[r]) \Omega'[r] \right) / \left( (\text{bz}^2 \text{Db}\phi^2 r^{2nz} (-3 m^2 r^2 + H^2 (m^2 + k^2 r^2))^2 - \right. \\
& \quad m^2 r^2 (3 \text{bz}^2 r^{2nz} (m^2 + k^2 r^2) + \text{Db}\phi^2 (-3 r^2 + H^2 (m^2 + k^2 r^2))) \sigma[r]^2 \Sigma[r] + \\
& \quad 3 m^4 r^4 \sigma[r]^4 \Sigma[r]^2 + c[r]^2 \Sigma[r] (-6 \text{bz} \text{Db}\phi k^2 m r^{3+nz} + 3 \text{bz}^2 k^2 r^{2+2nz} (m^2 + k^2 r^2) + \\
& \quad \text{Db}\phi^2 m^2 (-3 r^2 + H^2 (m^2 + k^2 r^2)) - 3 m^2 r^2 (m^2 + k^2 r^2) \sigma[r]^2 \Sigma[r]) \Omega[r]^2 + \\
& \quad \left. (3 \text{Db}\phi^2 H^2 k^2 m r^4 K^2[r] \Sigma[r] (\text{bz} \text{Db}\phi r^{1+nz} + m c[r]^2 \Sigma[r]) \Omega'[r]) \right) / \\
& \left( (\text{bz}^2 \text{Db}\phi^2 r^{2nz} (-3 m^2 r^2 + H^2 (m^2 + k^2 r^2))^2 - \right. \\
& \quad m^2 r^2 (3 \text{bz}^2 r^{2nz} (m^2 + k^2 r^2) + \text{Db}\phi^2 (-3 r^2 + H^2 (m^2 + k^2 r^2))) \sigma[r]^2 \Sigma[r] + \\
& \quad 3 m^4 r^4 \sigma[r]^4 \Sigma[r]^2 + c[r]^2 \Sigma[r] (-6 \text{bz} \text{Db}\phi k^2 m r^{3+nz} + 3 \text{bz}^2 k^2 r^{2+2nz} (m^2 + k^2 r^2) + \\
& \quad \text{Db}\phi^2 m^2 (-3 r^2 + H^2 (m^2 + k^2 r^2)) - 3 m^2 r^2 (m^2 + k^2 r^2) \sigma[r]^2 \Sigma[r]) \Omega[r] - \\
& \quad \left. (3 \text{bz}^2 m^2 r^{2+2nz} K^2[r] \Sigma[r] (\text{Db}\phi^2 (-3 r^2 + H^2 (m^2 + k^2 r^2)) + 3 k^2 r^2 c[r]^2 \Sigma[r] - \right. \\
& \quad \left. 3 m^2 r^2 \sigma[r]^2 \Sigma[r]) \Omega'[r] \right) / \left( (\text{bz}^2 \text{Db}\phi^2 r^{2nz} (-3 m^2 r^2 + H^2 (m^2 + k^2 r^2))^2 - \right. \\
& \quad m^2 r^2 (3 \text{bz}^2 r^{2nz} (m^2 + k^2 r^2) + \text{Db}\phi^2 (-3 r^2 + H^2 (m^2 + k^2 r^2))) \sigma[r]^2 \Sigma[r] + \\
& \quad 3 m^4 r^4 \sigma[r]^4 \Sigma[r]^2 + c[r]^2 \Sigma[r] (-6 \text{bz} \text{Db}\phi k^2 m r^{3+nz} + 3 \text{bz}^2 k^2 r^{2+2nz} (m^2 + k^2 r^2) + \\
& \quad \text{Db}\phi^2 m^2 (-3 r^2 + H^2 (m^2 + k^2 r^2)) - 3 m^2 r^2 (m^2 + k^2 r^2) \sigma[r]^2 \Sigma[r]) \Omega[r] + \\
& \quad \left. \frac{6 \text{bz}^2 r^{1+2nz} \Omega'[r]^2}{\sigma[r]^2} + (3 \text{bz}^2 m^2 r^{3+2nz} K^2[r] \sigma[r] \Sigma[r] (-2 \text{Db}\phi^2 (-3 + H^2 k^2) - \right. \\
& \quad \left. 6 k^2 r c[r] \Sigma[r] c'[r] - 3 k^2 c[r]^2 (2 \Sigma[r] + r \Sigma'[r]) + 3 m^2 \sigma[r]^2 (2 \Sigma[r] + r \Sigma'[r]) + \right. \\
& \quad \left. 6 m^2 r \sigma[r] \Sigma[r] \Omega'[r]) \right) / \left( (\text{bz}^2 \text{Db}\phi^2 r^{2nz} (-3 m^2 r^2 + H^2 (m^2 + k^2 r^2))^2 - \right. \\
& \quad m^2 r^2 (3 \text{bz}^2 r^{2nz} (m^2 + k^2 r^2) + \text{Db}\phi^2 (-3 r^2 + H^2 (m^2 + k^2 r^2))) \sigma[r]^2 \Sigma[r] + \\
& \quad 3 m^4 r^4 \sigma[r]^4 \Sigma[r]^2 + c[r]^2 \Sigma[r] (-6 \text{bz} \text{Db}\phi k^2 m r^{3+nz} + 3 \text{bz}^2 k^2 r^{2+2nz} (m^2 + k^2 r^2) + \\
& \quad \text{Db}\phi^2 m^2 (-3 r^2 + H^2 (m^2 + k^2 r^2)) - 3 m^2 r^2 (m^2 + k^2 r^2) \sigma[r]^2 \Sigma[r]) \Omega[r] - \\
& \quad \left. (2 \text{bz}^2 r^{2nz} \Sigma'[r] (-3 m^3 r^2 \sigma[r]^3 \Sigma[r] (3 m c[r]^2 \Sigma[r]^2 - 3 \text{bz} \text{Db}\phi r^{2+nz} \Sigma'[r] + \Sigma[r] \right. \\
& \quad \left. (\text{Db}\phi^2 H^2 m + 3 \text{bz}^2 m (1 + nz) r^{2nz} + 3 \text{bz} \text{Db}\phi nz r^{1+nz} + 3 m r c[r]^2 \Sigma'[r])) + m \sigma[r] \right. \\
& \quad \left. (3 (3 \text{bz} \text{Db}\phi k^2 (-1 + nz) r^{3+nz} + 3 \text{bz}^2 k^2 m r^{2+2nz} + \text{Db}\phi^2 m (-3 r^2 + H^2 (m^2 + 2 k^2 r^2))) \right. \\
& \quad \left. c[r]^2 \Sigma[r]^2 - 3 \text{bz} \text{Db}\phi^3 r^{2+nz} (-3 r^2 + H^2 (m^2 + k^2 r^2)) \Sigma'[r] + \text{Db}\phi \Sigma[r] \right. \\
& \quad \left. (-9 \text{bz}^3 k^2 nz r^{3+3nz} + \text{Db}\phi^3 H^2 m (-3 r^2 + H^2 (m^2 + k^2 r^2)) + 3 \text{bz}^2 \text{Db}\phi m (1 + nz) \right. \\
& \quad \left. r^{2nz} (-3 r^2 + H^2 (m^2 + k^2 r^2)) + 3 \text{bz} \text{Db}\phi^2 nz r^{1+nz} (-3 r^2 + H^2 (m^2 + k^2 r^2)) + \right. \\
& \quad \left. 3 r (-6 \text{bz} k^2 r^{3+nz} + \text{Db}\phi m (-3 r^2 + H^2 (m^2 + k^2 r^2))) c[r]^2 \Sigma'[r] \right) - \\
& \quad \left. 9 m^2 r^3 \sigma[r]^2 \Sigma[r]^2 (\text{bz}^2 r^{2nz} (m^2 + k^2 r^2) + m^2 c[r]^2 \Sigma[r]) \Omega'[r] + \right. \\
& \quad \left. 3 r \Sigma[r] (\text{bz}^2 \text{Db}\phi^2 r^{2nz} (-3 m^2 r^2 + H^2 (m^2 + k^2 r^2))^2 + (-6 \text{bz} \text{Db}\phi k^2 m r^{3+nz} + 3 \text{bz}^2 k^2 \right. \\
& \quad \left. r^{2+2nz} (m^2 + k^2 r^2) + \text{Db}\phi^2 m^2 (-3 r^2 + H^2 (m^2 + k^2 r^2))) c[r]^2 \Sigma[r] \Omega'[r] \right) / \\
& \left( \sigma[r] \Sigma[r]^2 (\text{bz}^2 \text{Db}\phi^2 r^{2nz} (-3 m^2 r^2 + H^2 (m^2 + k^2 r^2))^2 - m^2 r^2 (3 \text{bz}^2 r^{2nz} \right.
\end{aligned}$$

$$\begin{aligned}
& \left( m^2 + k^2 r^2 \right) + \text{Db}\phi^2 \left( -3 r^2 + H^2 \left( m^2 + k^2 r^2 \right) \right) \left( \sigma[r]^2 \Sigma[r] + 3 m^4 r^4 \sigma[r]^4 \Sigma[r]^2 + \right. \\
& \left. c[r]^2 \Sigma[r] \left( -6 i b z \text{Db}\phi k^2 m r^{3+nz} + 3 b z^2 k^2 r^{2+2nz} \left( m^2 + k^2 r^2 \right) + \text{Db}\phi^2 m^2 \right. \right. \\
& \left. \left. \left( -3 r^2 + H^2 \left( m^2 + k^2 r^2 \right) \right) - 3 m^2 r^2 \left( m^2 + k^2 r^2 \right) \sigma[r]^2 \Sigma[r] \right) \right) - \\
& \left( 2 b z^2 r^{2nz} \Omega'[r] \left( -3 m^3 r^2 \sigma[r]^3 \Sigma[r] \left( 3 m c[r]^2 \Sigma[r]^2 - 3 i b z \text{Db}\phi r^{2+nz} \Sigma'[r] + \Sigma[r] \right. \right. \right. \\
& \left. \left. \left( \text{Db}\phi^2 H^2 m + 3 b z^2 m (1+nz) r^{2nz} + 3 i b z \text{Db}\phi n z r^{1+nz} + 3 m r c[r]^2 \Sigma'[r] \right) \right) + m \sigma[r] \right. \\
& \left. \left( 3 \left( 3 i b z \text{Db}\phi k^2 (-1+nz) r^{3+nz} + 3 b z^2 k^2 m r^{2+2nz} + \text{Db}\phi^2 m \left( -3 r^2 + H^2 \left( m^2 + 2 k^2 r^2 \right) \right) \right) \right. \right. \\
& \left. \left. c[r]^2 \Sigma[r]^2 - 3 i b z \text{Db}\phi^3 r^{2+nz} \left( -3 r^2 + H^2 \left( m^2 + k^2 r^2 \right) \right) \Sigma'[r] + \text{Db}\phi \Sigma[r] \right. \right. \\
& \left. \left. \left( -9 i b z^3 k^2 n z r^{3+3nz} + \text{Db}\phi^3 H^2 m \left( -3 r^2 + H^2 \left( m^2 + k^2 r^2 \right) \right) + 3 b z^2 \text{Db}\phi m (1+nz) \right. \right. \right. \\
& \left. \left. \left. r^{2nz} \left( -3 r^2 + H^2 \left( m^2 + k^2 r^2 \right) \right) + 3 i b z \text{Db}\phi^2 n z r^{1+nz} \left( -3 r^2 + H^2 \left( m^2 + k^2 r^2 \right) \right) + \right. \right. \right. \\
& \left. \left. \left. 3 r \left( -6 i b z k^2 r^{3+nz} + \text{Db}\phi m \left( -3 r^2 + H^2 \left( m^2 + k^2 r^2 \right) \right) \right) c[r]^2 \Sigma'[r] \right) \right) - \right. \\
& \left. 9 m^2 r^3 \sigma[r]^2 \Sigma[r]^2 \left( b z^2 r^{2nz} \left( m^2 + k^2 r^2 \right) + m^2 c[r]^2 \Sigma[r] \right) \Omega'[r] + \right. \\
& \left. 3 r \Sigma[r] \left( b z^2 \text{Db}\phi^2 r^{2nz} \left( -3 m^2 r^2 + H^2 \left( m^2 + k^2 r^2 \right)^2 \right) + \left( -6 i b z \text{Db}\phi k^2 m r^{3+nz} + 3 b z^2 k^2 \right. \right. \right. \\
& \left. \left. \left. r^{2+2nz} \left( m^2 + k^2 r^2 \right) + \text{Db}\phi^2 m^2 \left( -3 r^2 + H^2 \left( m^2 + k^2 r^2 \right) \right) \right) c[r]^2 \Sigma[r] \right) \Omega'[r] \right) \Bigg/ \\
& \left( \sigma[r]^2 \Sigma[r] \left( b z^2 \text{Db}\phi^2 r^{2nz} \left( -3 m^2 r^2 + H^2 \left( m^2 + k^2 r^2 \right)^2 \right) - m^2 r^2 \left( 3 b z^2 r^{2nz} \right. \right. \right. \\
& \left. \left. \left. \left( m^2 + k^2 r^2 \right) + \text{Db}\phi^2 \left( -3 r^2 + H^2 \left( m^2 + k^2 r^2 \right) \right) \right) \sigma[r]^2 \Sigma[r] + 3 m^4 r^4 \sigma[r]^4 \Sigma[r]^2 + \right. \right. \\
& \left. \left. c[r]^2 \Sigma[r] \left( -6 i b z \text{Db}\phi k^2 m r^{3+nz} + 3 b z^2 k^2 r^{2+2nz} \left( m^2 + k^2 r^2 \right) + \text{Db}\phi^2 m^2 \right. \right. \right. \\
& \left. \left. \left. \left( -3 r^2 + H^2 \left( m^2 + k^2 r^2 \right) \right) - 3 m^2 r^2 \left( m^2 + k^2 r^2 \right) \sigma[r]^2 \Sigma[r] \right) \right) \right) - \\
& \left( 2 \text{Db}\phi^2 H^2 k^2 r \left( 3 b z^2 \text{Db}\phi^2 r^{3+2nz} \Sigma'[r] - b z r^{nz} \Sigma[r] \left( -i \text{Db}\phi^3 H^2 m r + 3 b z \text{Db}\phi^2 n z \right. \right. \right. \\
& \left. \left. \left. r^{2+nz} - 3 i b z^2 \text{Db}\phi m (1+nz) r^{1+2nz} + 3 b z^3 n z r^{3nz} \left( m^2 + k^2 r^2 \right) + 3 b z r^{1+nz} \right. \right. \right. \\
& \left. \left. \left. \left( m^2 + k^2 r^2 \right) c[r]^2 \Sigma'[r] \right) + 3 m^2 r^2 c[r]^2 \sigma[r] \Sigma[r]^3 \left( \sigma[r] + r \Omega'[r] \right) + \right. \right. \\
& \left. \left. \Sigma[r]^2 \left( c[r]^2 \left( \text{Db}\phi^2 H^2 m^2 + 3 i b z \text{Db}\phi m (1+nz) r^{1+nz} - 3 b z^2 k^2 r^{2+2nz} + \right. \right. \right. \right. \\
& \left. \left. \left. 3 m^2 r^3 \sigma[r]^2 \Sigma'[r] \right) + 3 b z m r^{2+nz} \sigma[r] \left( b z m n z r^{nz} \sigma[r] + i \text{Db}\phi r^2 \Omega'[r] \right) \right) \right) \Bigg/ \\
& \left( \Sigma[r] \left( b z^2 \text{Db}\phi^2 r^{2nz} \left( -3 m^2 r^2 + H^2 \left( m^2 + k^2 r^2 \right)^2 \right) - m^2 r^2 \left( 3 b z^2 r^{2nz} \left( m^2 + k^2 r^2 \right) + \right. \right. \right. \\
& \left. \left. \left. \text{Db}\phi^2 \left( -3 r^2 + H^2 \left( m^2 + k^2 r^2 \right) \right) \right) \sigma[r]^2 \Sigma[r] + 3 m^4 r^4 \sigma[r]^4 \Sigma[r]^2 + \right. \right. \\
& \left. \left. c[r]^2 \Sigma[r] \left( -6 i b z \text{Db}\phi k^2 m r^{3+nz} + 3 b z^2 k^2 r^{2+2nz} \left( m^2 + k^2 r^2 \right) + \text{Db}\phi^2 m^2 \right. \right. \right. \\
& \left. \left. \left. \left( -3 r^2 + H^2 \left( m^2 + k^2 r^2 \right) \right) - 3 m^2 r^2 \left( m^2 + k^2 r^2 \right) \sigma[r]^2 \Sigma[r] \right) \right) \right) + \\
& \left( 2 \text{Db}\phi^2 H^2 k^2 r^2 \Sigma'[r] \left( 3 b z^2 \text{Db}\phi^2 r^{3+2nz} \Sigma'[r] - b z r^{nz} \Sigma[r] \left( -i \text{Db}\phi^3 H^2 m r + 3 b z \right. \right. \right. \\
& \left. \left. \left. \text{Db}\phi^2 n z r^{2+nz} - 3 i b z^2 \text{Db}\phi m (1+nz) r^{1+2nz} + 3 b z^3 n z r^{3nz} \left( m^2 + k^2 r^2 \right) + 3 b z \right. \right. \right. \\
& \left. \left. \left. r^{1+nz} \left( m^2 + k^2 r^2 \right) c[r]^2 \Sigma'[r] \right) + 3 m^2 r^2 c[r]^2 \sigma[r] \Sigma[r]^3 \left( \sigma[r] + r \Omega'[r] \right) + \right. \right. \\
& \left. \left. \Sigma[r]^2 \left( c[r]^2 \left( \text{Db}\phi^2 H^2 m^2 + 3 i b z \text{Db}\phi m (1+nz) r^{1+nz} - 3 b z^2 k^2 r^{2+2nz} + \right. \right. \right. \right. \\
& \left. \left. \left. 3 m^2 r^3 \sigma[r]^2 \Sigma'[r] \right) + 3 b z m r^{2+nz} \sigma[r] \left( b z m n z r^{nz} \sigma[r] + i \text{Db}\phi r^2 \Omega'[r] \right) \right) \right) \Bigg/ \\
& \left( \Sigma[r]^2 \left( b z^2 \text{Db}\phi^2 r^{2nz} \left( -3 m^2 r^2 + H^2 \left( m^2 + k^2 r^2 \right)^2 \right) - m^2 r^2 \left( 3 b z^2 r^{2nz} \left( m^2 + k^2 r^2 \right) + \right. \right. \right. \\
& \left. \left. \left. \text{Db}\phi^2 \left( -3 r^2 + H^2 \left( m^2 + k^2 r^2 \right) \right) \right) \sigma[r]^2 \Sigma[r] + 3 m^4 r^4 \sigma[r]^4 \Sigma[r]^2 + \right. \right. \\
& \left. \left. c[r]^2 \Sigma[r] \left( -6 i b z \text{Db}\phi k^2 m r^{3+nz} + 3 b z^2 k^2 r^{2+2nz} \left( m^2 + k^2 r^2 \right) + \text{Db}\phi^2 m^2 \right. \right. \right. \\
& \left. \left. \left. \left( -3 r^2 + H^2 \left( m^2 + k^2 r^2 \right) \right) - 3 m^2 r^2 \left( m^2 + k^2 r^2 \right) \sigma[r]^2 \Sigma[r] \right) \right) \right) - \\
& \left( 3 i \text{Db}\phi^2 H^2 k^2 m r^3 K^2[r] \sigma[r] \Sigma[r] \left( b z \text{Db}\phi r^{1+nz} - i m c[r]^2 \Sigma[r] \right) \right. \\
& \left( 2 b z^2 \text{Db}\phi^2 r^{2nz} \left( -3 m^2 (1+nz) r^2 + H^2 \left( m^2 + k^2 r^2 \right) \left( m^2 n z + k^2 (2+nz) r^2 \right) \right) + 2 r c[r] \Sigma[r] \right. \\
& \left. \left( -6 i b z \text{Db}\phi k^2 m r^{3+nz} + 3 b z^2 k^2 r^{2+2nz} \left( m^2 + k^2 r^2 \right) + \text{Db}\phi^2 m^2 \left( -3 r^2 + H^2 \left( m^2 + k^2 r^2 \right) \right) - 3 \right. \right. \\
& \left. \left. m^2 r^2 \left( m^2 + k^2 r^2 \right) \sigma[r]^2 \Sigma[r] \right) c'[r] + 6 m^4 r^4 \sigma[r]^4 \Sigma[r] \left( 2 \Sigma[r] + r \Sigma'[r] \right) - \right. \\
& \left. m^2 r^2 \sigma[r]^2 \left( 2 \left( 3 b z^2 r^{2nz} \left( m^2 (1+nz) + k^2 (2+nz) r^2 \right) + \text{Db}\phi^2 \left( -6 r^2 + H^2 \left( m^2 + 2 k^2 r^2 \right) \right) \right) \right. \right. \\
& \left. \left. \Sigma[r] + r \left( 3 b z^2 r^{2nz} \left( m^2 + k^2 r^2 \right) + \text{Db}\phi^2 \left( -3 r^2 + H^2 \left( m^2 + k^2 r^2 \right) \right) \right) \Sigma'[r] \right) - \right. \\
& \left. 2 m^2 r^3 \left( 3 b z^2 r^{2nz} \left( m^2 + k^2 r^2 \right) + \text{Db}\phi^2 \left( -3 r^2 + H^2 \left( m^2 + k^2 r^2 \right) \right) \right) \sigma[r] \Sigma[r] \Omega'[r] + \right. \\
& \left. 12 m^4 r^5 \sigma[r]^3 \Sigma[r]^2 \Omega'[r] + r c[r]^2 \left( \left( -6 i b z \text{Db}\phi k^2 m r^{3+nz} + 3 b z^2 k^2 r^{2+2nz} \left( m^2 + k^2 r^2 \right) + \right. \right. \right. \\
& \left. \left. \left. \text{Db}\phi^2 m^2 \left( -3 r^2 + H^2 \left( m^2 + k^2 r^2 \right) \right) \right) \Sigma'[r] + 2 r \Sigma[r] \left( \text{Db}\phi^2 \left( -3 + H^2 k^2 \right) m^2 - 3 i b z \text{Db}\phi \right. \right. \right. \\
& \left. \left. \left. k^2 m (3+nz) r^{1+nz} + 3 b z^2 k^2 r^{2nz} \left( m^2 (1+nz) + k^2 (2+nz) r^2 \right) - 3 m^2 r \left( m^2 + k^2 r^2 \right) \right. \right. \right. \\
& \left. \left. \left. \sigma[r]^2 \Sigma'[r] \right) - 6 m^2 r \sigma[r] \Sigma[r]^2 \left( \left( m^2 + 2 k^2 r^2 \right) \sigma[r] + r \left( m^2 + k^2 r^2 \right) \Omega'[r] \right) \right) \right) \Bigg/
\end{aligned}$$

$$\begin{aligned}
& \left( (b z^2 D b \phi^2 r^{2 n z} (-3 m^2 r^2 + H^2 (m^2 + k^2 r^2)^2) - m^2 r^2 (3 b z^2 r^{2 n z} (m^2 + k^2 r^2) + \right. \\
& \quad D b \phi^2 (-3 r^2 + H^2 (m^2 + k^2 r^2))) \sigma[r]^2 \Sigma[r] + 3 m^4 r^4 \sigma[r]^4 \Sigma[r]^2 + \\
& \quad c[r]^2 \Sigma[r] (-6 i b z D b \phi k^2 m r^{3+n z} + 3 b z^2 k^2 r^{2+2 n z} (m^2 + k^2 r^2) + \\
& \quad D b \phi^2 m^2 (-3 r^2 + H^2 (m^2 + k^2 r^2)) - 3 m^2 r^2 (m^2 + k^2 r^2) \sigma[r]^2 \Sigma[r]) \left. \right)^2 \Omega[r] \Big) + \\
& (2 D b \phi^2 H^2 k^2 r (3 b z^2 D b \phi^2 r^{3+2 n z} \Sigma'[r] - b z r^{n z} \Sigma[r] (-i D b \phi^3 H^2 m r + 3 b z D b \phi^2 n z \\
& \quad r^{2+n z} - 3 i b z^2 D b \phi m (1+n z) r^{1+2 n z} + 3 b z^3 n z r^{3 n z} (m^2 + k^2 r^2) + 3 b z r^{1+n z} \\
& \quad (m^2 + k^2 r^2) c[r]^2 \Sigma'[r]) + 3 m^2 r^2 c[r]^2 \sigma[r] \Sigma[r]^3 (\sigma[r] + r \Omega'[r]) + \\
& \quad \Sigma[r]^2 (c[r]^2 (D b \phi^2 H^2 m^2 + 3 i b z D b \phi m (1+n z) r^{1+n z} - 3 b z^2 k^2 r^{2+2 n z} + \\
& \quad 3 m^2 r^3 \sigma[r]^2 \Sigma'[r]) + 3 b z m r^{2+n z} \sigma[r] (b z m n z r^{n z} \sigma[r] + i D b \phi r^2 \Omega'[r])) \Big) \\
& (2 b z^2 D b \phi^2 r^{2 n z} (-3 m^2 (1+n z) r^2 + H^2 (m^2 + k^2 r^2) (m^2 n z + k^2 (2+n z) r^2)) + 2 r c[r] \Sigma[r] \\
& \quad (-6 i b z D b \phi k^2 m r^{3+n z} + 3 b z^2 k^2 r^{2+2 n z} (m^2 + k^2 r^2) + D b \phi^2 m^2 (-3 r^2 + H^2 (m^2 + k^2 r^2)) - 3 \\
& \quad m^2 r^2 (m^2 + k^2 r^2) \sigma[r]^2 \Sigma[r]) c'[r] + 6 m^4 r^4 \sigma[r]^4 \Sigma[r] (2 \Sigma[r] + r \Sigma'[r]) - \\
& \quad m^2 r^2 \sigma[r]^2 (2 (3 b z^2 r^{2 n z} (m^2 (1+n z) + k^2 (2+n z) r^2) + D b \phi^2 (-6 r^2 + H^2 (m^2 + 2 k^2 r^2))) \\
& \quad \Sigma[r] + r (3 b z^2 r^{2 n z} (m^2 + k^2 r^2) + D b \phi^2 (-3 r^2 + H^2 (m^2 + k^2 r^2))) \Sigma'[r]) - \\
& \quad 2 m^2 r^3 (3 b z^2 r^{2 n z} (m^2 + k^2 r^2) + D b \phi^2 (-3 r^2 + H^2 (m^2 + k^2 r^2))) \sigma[r] \Sigma[r] \Omega'[r] + \\
& \quad 12 m^4 r^5 \sigma[r]^3 \Sigma[r]^2 \Omega'[r] + r c[r]^2 ((-6 i b z D b \phi k^2 m r^{3+n z} + 3 b z^2 k^2 r^{2+2 n z} (m^2 + k^2 r^2) + \\
& \quad D b \phi^2 m^2 (-3 r^2 + H^2 (m^2 + k^2 r^2))) \Sigma'[r] + 2 r \Sigma[r] (D b \phi^2 (-3 + H^2 k^2) m^2 - 3 i b z D b \phi \\
& \quad k^2 m (3+n z) r^{1+n z} + 3 b z^2 k^2 r^{2 n z} (m^2 (1+n z) + k^2 (2+n z) r^2) - 3 m^2 r (m^2 + k^2 r^2) \\
& \quad \sigma[r]^2 \Sigma'[r]) - 6 m^2 r \sigma[r] \Sigma[r]^2 ((m^2 + 2 k^2 r^2) \sigma[r] + r (m^2 + k^2 r^2) \Omega'[r])) \Big) \Big) / \\
& \left( \Sigma[r] (b z^2 D b \phi^2 r^{2 n z} (-3 m^2 r^2 + H^2 (m^2 + k^2 r^2)^2) - m^2 r^2 (3 b z^2 r^{2 n z} (m^2 + k^2 r^2) + \right. \\
& \quad D b \phi^2 (-3 r^2 + H^2 (m^2 + k^2 r^2))) \sigma[r]^2 \Sigma[r] + 3 m^4 r^4 \sigma[r]^4 \Sigma[r]^2 + \\
& \quad c[r]^2 \Sigma[r] (-6 i b z D b \phi k^2 m r^{3+n z} + 3 b z^2 k^2 r^{2+2 n z} (m^2 + k^2 r^2) + \\
& \quad D b \phi^2 m^2 (-3 r^2 + H^2 (m^2 + k^2 r^2)) - 3 m^2 r^2 (m^2 + k^2 r^2) \sigma[r]^2 \Sigma[r]) \left. \right)^2 \Big) + \\
& (3 b z^2 m^2 r^{1+2 n z} K^2[r] \sigma[r] \Sigma[r] (-D b \phi^2 (-3 r^2 + H^2 (m^2 + k^2 r^2)) - 3 k^2 r^2 c[r]^2 \Sigma[r] + \\
& \quad 3 m^2 r^2 \sigma[r]^2 \Sigma[r]) \\
& \quad (-2 b z^2 D b \phi^2 r^{2 n z} (-3 m^2 (1+n z) r^2 + H^2 (m^2 + k^2 r^2) (m^2 n z + k^2 (2+n z) r^2)) - 2 r c[r] \Sigma[r] \\
& \quad (-6 i b z D b \phi k^2 m r^{3+n z} + 3 b z^2 k^2 r^{2+2 n z} (m^2 + k^2 r^2) + D b \phi^2 m^2 (-3 r^2 + H^2 (m^2 + k^2 r^2)) - 3 \\
& \quad m^2 r^2 (m^2 + k^2 r^2) \sigma[r]^2 \Sigma[r]) c'[r] - 6 m^4 r^4 \sigma[r]^4 \Sigma[r] (2 \Sigma[r] + r \Sigma'[r]) + \\
& \quad m^2 r^2 \sigma[r]^2 (2 (3 b z^2 r^{2 n z} (m^2 (1+n z) + k^2 (2+n z) r^2) + D b \phi^2 (-6 r^2 + H^2 (m^2 + 2 k^2 r^2))) \\
& \quad \Sigma[r] + r (3 b z^2 r^{2 n z} (m^2 + k^2 r^2) + D b \phi^2 (-3 r^2 + H^2 (m^2 + k^2 r^2))) \Sigma'[r]) + \\
& \quad 2 m^2 r^3 (3 b z^2 r^{2 n z} (m^2 + k^2 r^2) + D b \phi^2 (-3 r^2 + H^2 (m^2 + k^2 r^2))) \sigma[r] \Sigma[r] \Omega'[r] - \\
& \quad 12 m^4 r^5 \sigma[r]^3 \Sigma[r]^2 \Omega'[r] + r c[r]^2 ((6 i b z D b \phi k^2 m r^{3+n z} - 3 b z^2 k^2 r^{2+2 n z} (m^2 + k^2 r^2) - \\
& \quad D b \phi^2 m^2 (-3 r^2 + H^2 (m^2 + k^2 r^2))) \Sigma'[r] + 2 r \Sigma[r] (D b \phi^2 (3 - H^2 k^2) m^2 + 3 i b z D b \phi \\
& \quad k^2 m (3+n z) r^{1+n z} - 3 b z^2 k^2 r^{2 n z} (m^2 (1+n z) + k^2 (2+n z) r^2) + 3 m^2 r (m^2 + k^2 r^2) \\
& \quad \sigma[r]^2 \Sigma'[r]) + 6 m^2 r \sigma[r] \Sigma[r]^2 ((m^2 + 2 k^2 r^2) \sigma[r] + r (m^2 + k^2 r^2) \Omega'[r])) \Big) \Big) / \\
& \left( (b z^2 D b \phi^2 r^{2 n z} (-3 m^2 r^2 + H^2 (m^2 + k^2 r^2)^2) - m^2 r^2 (3 b z^2 r^{2 n z} (m^2 + k^2 r^2) + \right. \\
& \quad D b \phi^2 (-3 r^2 + H^2 (m^2 + k^2 r^2))) \sigma[r]^2 \Sigma[r] + 3 m^4 r^4 \sigma[r]^4 \Sigma[r]^2 + \\
& \quad c[r]^2 \Sigma[r] (-6 i b z D b \phi k^2 m r^{3+n z} + 3 b z^2 k^2 r^{2+2 n z} (m^2 + k^2 r^2) + \\
& \quad D b \phi^2 m^2 (-3 r^2 + H^2 (m^2 + k^2 r^2)) - 3 m^2 r^2 (m^2 + k^2 r^2) \sigma[r]^2 \Sigma[r]) \left. \right)^2 \Omega[r] \Big) + \\
& (2 b z^2 r^{-1+2 n z} (-3 m^3 r^2 \sigma[r]^3 \Sigma[r] (3 m c[r]^2 \Sigma[r]^2 - 3 i b z D b \phi r^{2+n z} \Sigma'[r] + \Sigma[r] \\
& \quad (D b \phi^2 H^2 m + 3 b z^2 m (1+n z) r^{2 n z} + 3 i b z D b \phi n z r^{1+n z} + 3 m r c[r]^2 \Sigma'[r])) + m \sigma[r] \\
& \quad (3 (3 i b z D b \phi k^2 (-1+n z) r^{3+n z} + 3 b z^2 k^2 m r^{2+2 n z} + D b \phi^2 m (-3 r^2 + H^2 (m^2 + 2 k^2 r^2))) \\
& \quad c[r]^2 \Sigma[r]^2 - 3 i b z D b \phi^3 r^{2+n z} (-3 r^2 + H^2 (m^2 + k^2 r^2)) \Sigma'[r] + D b \phi \Sigma[r] \\
& \quad (-9 i b z^3 k^2 n z r^{3+3 n z} + D b \phi^3 H^2 m (-3 r^2 + H^2 (m^2 + k^2 r^2)) + 3 b z^2 D b \phi m (1+n z)
\end{aligned}$$

$$\begin{aligned}
& r^{2nz} \left( -3r^2 + H^2 (m^2 + k^2 r^2) \right) + 3 \, i \, bz \, Db\phi^2 \, nz \, r^{1+nz} \left( -3r^2 + H^2 (m^2 + k^2 r^2) \right) + \\
& 3r \left( -6 \, i \, bz \, k^2 \, r^{3+nz} + Db\phi \, m \left( -3r^2 + H^2 (m^2 + k^2 r^2) \right) \right) c[r]^2 \, \Sigma'[r] - \\
& 9m^2 r^3 \, \sigma[r]^2 \, \Sigma[r]^2 \left( bz^2 r^{2nz} (m^2 + k^2 r^2) + m^2 c[r]^2 \, \Sigma[r] \right) \Omega'[r] + \\
& 3r \, \Sigma[r] \left( bz^2 \, Db\phi^2 \, r^{2nz} \left( -3m^2 r^2 + H^2 (m^2 + k^2 r^2)^2 \right) + \left( -6 \, i \, bz \, Db\phi \, k^2 \, m \, r^{3+nz} + \right. \right. \\
& \quad \left. \left. 3bz^2 k^2 r^{2+2nz} (m^2 + k^2 r^2) + Db\phi^2 m^2 \left( -3r^2 + H^2 (m^2 + k^2 r^2) \right) \right) \right) c[r]^2 \, \Sigma[r] \, \Omega'[r] + \\
& \left( -2bz^2 \, Db\phi^2 \, r^{2nz} \left( -3m^2 (1+nz) r^2 + H^2 (m^2 + k^2 r^2) (m^2 nz + k^2 (2+nz) r^2) \right) - 2r \, c[r] \, \Sigma[r] \right. \\
& \quad \left( -6 \, i \, bz \, Db\phi \, k^2 \, m \, r^{3+nz} + 3bz^2 k^2 r^{2+2nz} (m^2 + k^2 r^2) + Db\phi^2 m^2 \left( -3r^2 + H^2 (m^2 + k^2 r^2) \right) - 3 \right. \\
& \quad \left. m^2 r^2 (m^2 + k^2 r^2) \sigma[r]^2 \, \Sigma[r] \right) c'[r] - 6m^4 r^4 \, \sigma[r]^4 \, \Sigma[r] \left( 2 \, \Sigma[r] + r \, \Sigma'[r] \right) + \\
& m^2 r^2 \, \sigma[r]^2 \left( 2 \left( 3bz^2 r^{2nz} (m^2 (1+nz) + k^2 (2+nz) r^2) + Db\phi^2 \left( -6r^2 + H^2 (m^2 + 2k^2 r^2) \right) \right) \right. \\
& \quad \left. \Sigma[r] + r \left( 3bz^2 r^{2nz} (m^2 + k^2 r^2) + Db\phi^2 \left( -3r^2 + H^2 (m^2 + k^2 r^2) \right) \right) \Sigma'[r] \right) + \\
& 2m^2 r^3 \left( 3bz^2 r^{2nz} (m^2 + k^2 r^2) + Db\phi^2 \left( -3r^2 + H^2 (m^2 + k^2 r^2) \right) \right) \sigma[r] \, \Sigma[r] \, \Omega'[r] - \\
& 12m^4 r^5 \, \sigma[r]^3 \, \Sigma[r]^2 \, \Omega'[r] + r \, c[r]^2 \left( \left( 6 \, i \, bz \, Db\phi \, k^2 \, m \, r^{3+nz} - 3bz^2 k^2 r^{2+2nz} (m^2 + k^2 r^2) - \right. \right. \\
& \quad \left. \left. Db\phi^2 m^2 \left( -3r^2 + H^2 (m^2 + k^2 r^2) \right) \right) \Sigma'[r] + 2r \, \Sigma[r] \left( Db\phi^2 \left( 3 - H^2 k^2 \right) m^2 + 3 \, i \, bz \, Db\phi \right. \right. \\
& \quad \left. \left. k^2 \, m \left( 3+nz \right) r^{1+nz} - 3bz^2 k^2 r^{2nz} (m^2 (1+nz) + k^2 (2+nz) r^2) + 3m^2 r (m^2 + k^2 r^2) \right. \right. \\
& \quad \left. \left. \sigma[r]^2 \, \Sigma'[r] \right) + 6m^2 r \, \sigma[r] \, \Sigma[r]^2 \left( (m^2 + 2k^2 r^2) \sigma[r] + r (m^2 + k^2 r^2) \Omega'[r] \right) \right) \Bigg) / \\
& \left( \sigma[r] \, \Sigma[r] \left( bz^2 \, Db\phi^2 \, r^{2nz} \left( -3m^2 r^2 + H^2 (m^2 + k^2 r^2)^2 \right) - m^2 r^2 \left( 3bz^2 r^{2nz} (m^2 + k^2 r^2) + \right. \right. \right. \\
& \quad \left. \left. Db\phi^2 \left( -3r^2 + H^2 (m^2 + k^2 r^2) \right) \right) \sigma[r]^2 \, \Sigma[r] + 3m^4 r^4 \, \sigma[r]^4 \, \Sigma[r]^2 + \right. \\
& \quad \left. c[r]^2 \, \Sigma[r] \left( -6 \, i \, bz \, Db\phi \, k^2 \, m \, r^{3+nz} + 3bz^2 k^2 r^{2+2nz} (m^2 + k^2 r^2) + \right. \right. \\
& \quad \left. \left. Db\phi^2 m^2 \left( -3r^2 + H^2 (m^2 + k^2 r^2) \right) - 3m^2 r^2 (m^2 + k^2 r^2) \sigma[r]^2 \, \Sigma[r] \right) \right)^2 - \\
& \frac{6bz^2 r^{1+2nz} \Omega''[r]}{\sigma[r]} - \left( 2 \, Db\phi^2 \, H^2 \, k^2 \, r \left( -bz \, r^{1+nz} \left( (-i \, Db\phi^3 \, H^2 \, m \, r - 3bz \, Db\phi^2 (3+nz) \right. \right. \right. \\
& \quad \left. \left. r^{2+nz} - 3 \, i \, bz^2 \, Db\phi \, m (1+nz) r^{1+2nz} + 3bz^3 \, nz \, r^{3nz} (m^2 + k^2 r^2) \right) \right. \\
& \quad \left. \Sigma'[r] + 3bz \, r^{1+nz} (m^2 + k^2 r^2) c[r]^2 \, \Sigma'[r]^2 - 3bz \, Db\phi^2 \, r^{3+nz} \Sigma''[r] \right) - \\
& \Sigma[r] \left( 6bz^2 r^{2+2nz} (m^2 + k^2 r^2) c[r] \, c'[r] \, \Sigma'[r] + bz \, r^{nz} \left( -i \, Db\phi^3 \, H^2 \, m (1+nz) r + \right. \right. \\
& \quad \left. \left. 6bz \, Db\phi^2 \, nz (1+nz) r^{2+nz} - 3 \, i \, bz^2 \, Db\phi \, m (1+4nz+3nz^2) r^{1+2nz} + \right. \right. \\
& \quad \left. \left. 6bz^3 \, nz \, r^{3nz} \left( 2m^2 nz + k^2 (1+2nz) r^2 \right) - 6bz \, m^2 \, nz \, r^{3+nz} \sigma[r]^2 \, \Sigma'[r] - 6 \, i \, Db\phi \right. \right. \\
& \quad \left. \left. m \, r^5 \sigma[r] \, \Sigma'[r] \, \Omega'[r] \right) - r \, c[r]^2 \left( \left( 2 \, Db\phi^2 \, H^2 \, m^2 + 6 \, i \, bz \, Db\phi \, m (1+nz) r^{1+nz} - \right. \right. \\
& \quad \left. \left. 3bz^2 r^{2nz} (m^2 (1+2nz) + k^2 (5+2nz) r^2) \right) \Sigma'[r] + 6m^2 r^3 \sigma[r]^2 \, \Sigma'[r]^2 - \right. \\
& \quad \left. 3bz^2 r^{1+2nz} (m^2 + k^2 r^2) \Sigma''[r] \right) + 3m^2 r^2 c[r] \, \Sigma[r]^3 \left( 2r \sigma[r] \, c'[r] \right. \\
& \quad \left. (\sigma[r] + r \Omega'[r]) + c[r] \left( 2 \sigma[r]^2 + r^2 \Omega'[r]^2 + r \sigma[r] (5 \Omega'[r] + r \Omega''[r]) \right) \right) + \\
& r \, \Sigma[r]^2 \left( 2 c[r] \, c'[r] \left( Db\phi^2 \, H^2 \, m^2 + 3 \, i \, bz \, Db\phi \, m (1+nz) r^{1+nz} - 3bz^2 k^2 r^{2+2nz} + \right. \right. \\
& \quad \left. \left. 3m^2 r^3 \sigma[r]^2 \, \Sigma'[r] \right) + 3 c[r]^2 \left( -bz (1+nz) r^{nz} \left( -i \, Db\phi \, m (1+nz) + 2bz \, k^2 \, r^{1+nz} \right) + \right. \right. \\
& \quad \left. \left. 5m^2 r^3 \sigma[r] \, \Sigma'[r] \, \Omega'[r] + m^2 r^2 \sigma[r]^2 (6 \Sigma'[r] + r \Sigma''[r]) \right) + 3 \right. \\
& \quad \left. bz \, m \, r^{1+nz} \left( 2bz \, m \, nz (1+nz) r^{nz} \sigma[r]^2 + i \, Db\phi \, r^3 \Omega'[r]^2 + \right. \right. \\
& \quad \left. \left. r \sigma[r] \left( (i \, Db\phi (4+nz) r + 2bz \, m \, nz \, r^{nz}) \Omega'[r] + i \, Db\phi \, r^2 \Omega''[r] \right) \right) \right) \Bigg) / \\
& \left( \Sigma[r] \left( bz^2 \, Db\phi^2 \, r^{2nz} \left( -3m^2 r^2 + H^2 (m^2 + k^2 r^2)^2 \right) - m^2 r^2 \left( 3bz^2 r^{2nz} (m^2 + k^2 r^2) + \right. \right. \right. \\
& \quad \left. \left. Db\phi^2 \left( -3r^2 + H^2 (m^2 + k^2 r^2) \right) \right) \sigma[r]^2 \, \Sigma[r] + 3m^4 r^4 \, \sigma[r]^4 \, \Sigma[r]^2 + \right. \\
& \quad \left. c[r]^2 \, \Sigma[r] \left( -6 \, i \, bz \, Db\phi \, k^2 \, m \, r^{3+nz} + 3bz^2 k^2 r^{2+2nz} (m^2 + k^2 r^2) + Db\phi^2 m^2 \right. \right. \\
& \quad \left. \left. \left( -3r^2 + H^2 (m^2 + k^2 r^2) \right) - 3m^2 r^2 (m^2 + k^2 r^2) \sigma[r]^2 \, \Sigma[r] \right) \right) + \\
& \left( 2bz^2 r^{-1+2nz} \left( -3m^3 r^2 \sigma[r]^3 \left( 6m c[r] \, \Sigma[r]^3 (c[r] + r c'[r]) - 3 \, i \, bz \, Db\phi \, r^{3+nz} \right. \right. \right. \\
& \quad \left. \left. \Sigma'[r]^2 + r \Sigma[r] \left( \left( 2 \, Db\phi^2 \, H^2 \, m + 6bz^2 \, m (1+nz) r^{2nz} + 3 \, i \, bz \, Db\phi \left( -4+nz \right) r^{1+nz} \right) \right. \right. \right. \\
& \quad \left. \left. \Sigma'[r] + 6m r \, c[r]^2 \, \Sigma'[r]^2 - 3 \, i \, bz \, Db\phi \, r^{2+nz} \Sigma''[r] \right) + \Sigma[r]^2 \right. \\
& \quad \left. \left( 2 \, Db\phi^2 \, H^2 \, m + 6bz^2 \, m (1+nz)^2 r^{2nz} + 3 \, i \, bz \, Db\phi \, nz (3+nz) r^{1+nz} + \right. \right. \\
& \quad \left. \left. 6m r^2 c[r] \, c'[r] \, \Sigma'[r] + 3m r \, c[r]^2 (6 \Sigma'[r] + r \Sigma''[r]) \right) \right) + \\
& m \sigma[r] \left( -18m^3 r^4 c[r]^2 \, \Sigma[r]^3 \, \Omega'[r]^2 + 3r \, \Sigma[r]^2 \left( r \left( 2 \, Db\phi^2 \left( -3+2H^2 k^2 \right) m + \right. \right. \right.
\end{aligned}$$

$$\begin{aligned} & 6 \mathbf{b} z^2 \mathbf{k}^2 \mathbf{m} (1 + \mathbf{n} z) \mathbf{r}^{2 \mathbf{n} z} + 3 \mathbf{i} \mathbf{b} z \mathbf{D} \mathbf{b} \phi \mathbf{k}^2 (-3 + 2 \mathbf{n} z + \mathbf{n} z^2) \mathbf{r}^{1 + \mathbf{n} z} \big) \mathbf{c} [\mathbf{r}]^2 + \\ & 2 \big( 3 \mathbf{i} \mathbf{b} z \mathbf{D} \mathbf{b} \phi \mathbf{k}^2 (-1 + \mathbf{n} z) \mathbf{r}^{3 + \mathbf{n} z} + 3 \mathbf{b} z^2 \mathbf{k}^2 \mathbf{m} \mathbf{r}^{2 + 2 \mathbf{n} z} + \mathbf{D} \mathbf{b} \phi^2 \mathbf{m} (-3 \mathbf{r}^2 + \\ & \quad \mathbf{H}^2 (\mathbf{m}^2 + 2 \mathbf{k}^2 \mathbf{r}^2)) \big) \mathbf{c} [\mathbf{r}] \mathbf{c}' [\mathbf{r}] - 6 \mathbf{b} z^2 \mathbf{m} \mathbf{r}^{3 + 2 \mathbf{n} z} (\mathbf{m}^2 + \mathbf{k}^2 \mathbf{r}^2) \Omega' [\mathbf{r}]^2 + \mathbf{D} \mathbf{b} \phi \mathbf{r} \\ & \big( (-9 \mathbf{i} \mathbf{b} z^3 \mathbf{k}^2 \mathbf{n} z \mathbf{r}^{3 + 3 \mathbf{n} z} + \mathbf{D} \mathbf{b} \phi^3 \mathbf{H}^2 \mathbf{m} (-3 \mathbf{r}^2 + \mathbf{H}^2 (\mathbf{m}^2 + \mathbf{k}^2 \mathbf{r}^2)) + 3 \mathbf{b} z^2 \mathbf{D} \mathbf{b} \phi \mathbf{m} (1 + \mathbf{n} z) \\ & \quad \mathbf{r}^{2 \mathbf{n} z} (-3 \mathbf{r}^2 + \mathbf{H}^2 (\mathbf{m}^2 + \mathbf{k}^2 \mathbf{r}^2)) - 6 \mathbf{i} \mathbf{b} z \mathbf{D} \mathbf{b} \phi^2 \mathbf{r}^{1 + \mathbf{n} z} (-6 \mathbf{r}^2 + \mathbf{H}^2 (\mathbf{m}^2 + 2 \mathbf{k}^2 \mathbf{r}^2)) \big) \\ & \quad \Sigma' [\mathbf{r}] + 3 \mathbf{r} (-6 \mathbf{i} \mathbf{b} z \mathbf{k}^2 \mathbf{r}^{3 + \mathbf{n} z} + \mathbf{D} \mathbf{b} \phi \mathbf{m} (-3 \mathbf{r}^2 + \mathbf{H}^2 (\mathbf{m}^2 + \mathbf{k}^2 \mathbf{r}^2)) \big) \mathbf{c} [\mathbf{r}]^2 \\ & \quad \Sigma' [\mathbf{r}]^2 - 3 \mathbf{i} \mathbf{b} z \mathbf{D} \mathbf{b} \phi^2 \mathbf{r}^{2 + \mathbf{n} z} (-3 \mathbf{r}^2 + \mathbf{H}^2 (\mathbf{m}^2 + \mathbf{k}^2 \mathbf{r}^2)) \Sigma'' [\mathbf{r}] + \Sigma [\mathbf{r}] \\ & \big( \mathbf{D} \mathbf{b} \phi (2 \mathbf{D} \mathbf{b} \phi^3 \mathbf{H}^2 (-3 + \mathbf{H}^2 \mathbf{k}^2) \mathbf{m} \mathbf{r}^2 - 27 \mathbf{i} \mathbf{b} z^3 \mathbf{k}^2 \mathbf{n} z (1 + \mathbf{n} z) \mathbf{r}^{3 + 3 \mathbf{n} z} + \\ & \quad 6 \mathbf{b} z^2 \mathbf{D} \mathbf{b} \phi \mathbf{m} (1 + \mathbf{n} z) \mathbf{r}^{2 \mathbf{n} z} (-3 (1 + \mathbf{n} z) \mathbf{r}^2 + \mathbf{H}^2 (\mathbf{m}^2 \mathbf{n} z + \mathbf{k}^2 (1 + \mathbf{n} z) \mathbf{r}^2)) + \\ & \quad 3 \mathbf{i} \mathbf{b} z \mathbf{D} \mathbf{b} \phi^2 \mathbf{n} z \mathbf{r}^{1 + \mathbf{n} z} (-3 (3 + \mathbf{n} z) \mathbf{r}^2 + \mathbf{H}^2 (\mathbf{m}^2 (1 + \mathbf{n} z) + \mathbf{k}^2 (3 + \mathbf{n} z) \mathbf{r}^2)) \big) + 6 \mathbf{D} \mathbf{b} \phi \\ & \quad \mathbf{r}^2 (-6 \mathbf{i} \mathbf{b} z \mathbf{k}^2 \mathbf{r}^{3 + \mathbf{n} z} + \mathbf{D} \mathbf{b} \phi \mathbf{m} (-3 \mathbf{r}^2 + \mathbf{H}^2 (\mathbf{m}^2 + \mathbf{k}^2 \mathbf{r}^2)) \big) \mathbf{c} [\mathbf{r}] \mathbf{c}' [\mathbf{r}] \Sigma' [\mathbf{r}] + 3 \mathbf{r} \mathbf{c} [\mathbf{r}]^2 \\ & \quad \big( (-30 \mathbf{i} \mathbf{b} z \mathbf{D} \mathbf{b} \phi \mathbf{k}^2 \mathbf{r}^{3 + \mathbf{n} z} + 6 \mathbf{b} z^2 \mathbf{k}^2 \mathbf{m} \mathbf{r}^{2 + 2 \mathbf{n} z} + \mathbf{D} \mathbf{b} \phi^2 \mathbf{m} (-15 \mathbf{r}^2 + \mathbf{H}^2 (3 \mathbf{m}^2 + 7 \mathbf{k}^2 \mathbf{r}^2)) \big) \\ & \quad \Sigma' [\mathbf{r}] + \mathbf{D} \mathbf{b} \phi \mathbf{r} (-6 \mathbf{i} \mathbf{b} z \mathbf{k}^2 \mathbf{r}^{3 + \mathbf{n} z} + \mathbf{D} \mathbf{b} \phi \mathbf{m} (-3 \mathbf{r}^2 + \mathbf{H}^2 (\mathbf{m}^2 + \mathbf{k}^2 \mathbf{r}^2)) \big) \Sigma'' [\mathbf{r}] \big) \big) - \\ & 9 \mathbf{m}^2 \mathbf{r}^3 \sigma [\mathbf{r}]^2 \Sigma [\mathbf{r}] \big( \mathbf{b} z \mathbf{r}^{1 + \mathbf{n} z} (-3 \mathbf{i} \mathbf{D} \mathbf{b} \phi \mathbf{m} \mathbf{r} + 2 \mathbf{b} z \mathbf{r}^{\mathbf{n} z} (\mathbf{m}^2 + \mathbf{k}^2 \mathbf{r}^2)) \Sigma' [\mathbf{r}] \Omega' [\mathbf{r}] + \\ & \quad \Sigma [\mathbf{r}] \big( (\mathbf{D} \mathbf{b} \phi^2 \mathbf{H}^2 \mathbf{m}^2 + 3 \mathbf{i} \mathbf{b} z \mathbf{D} \mathbf{b} \phi \mathbf{m} \mathbf{n} z \mathbf{r}^{1 + \mathbf{n} z} + \mathbf{b} z^2 \mathbf{r}^{2 \mathbf{n} z} (\mathbf{m}^2 (6 + 5 \mathbf{n} z) + \mathbf{k}^2 (5 + 2 \mathbf{n} z) \mathbf{r}^2) + \\ & \quad 6 \mathbf{m}^2 \mathbf{r} \mathbf{c} [\mathbf{r}]^2 \Sigma' [\mathbf{r}]) \Omega' [\mathbf{r}] + \mathbf{b} z^2 \mathbf{r}^{1 + 2 \mathbf{n} z} (\mathbf{m}^2 + \mathbf{k}^2 \mathbf{r}^2) \Omega'' [\mathbf{r}] + \mathbf{m}^2 \mathbf{c} [\mathbf{r}] \Sigma [\mathbf{r}]^2 \\ & \quad (2 \mathbf{r} \mathbf{c}' [\mathbf{r}] \Omega' [\mathbf{r}] + \mathbf{c} [\mathbf{r}] (6 \Omega' [\mathbf{r}] + \mathbf{r} \Omega'' [\mathbf{r}])) \big) + \mathbf{r} \big( 3 \mathbf{b} z \mathbf{D} \mathbf{b} \phi^2 \mathbf{r}^{1 + \mathbf{n} z} (-\mathbf{i} \mathbf{D} \mathbf{b} \phi \mathbf{m} \mathbf{r} \\ & \quad (-3 \mathbf{r}^2 + \mathbf{H}^2 (\mathbf{m}^2 + \mathbf{k}^2 \mathbf{r}^2)) + \mathbf{b} z \mathbf{r}^{\mathbf{n} z} (-3 \mathbf{m}^2 \mathbf{r}^2 + \mathbf{H}^2 (\mathbf{m}^2 + \mathbf{k}^2 \mathbf{r}^2)^2) \big) \Sigma' [\mathbf{r}] \Omega' [\mathbf{r}] + \Sigma [\mathbf{r}] \\ & \quad \big( (\mathbf{D} \mathbf{b} \phi (-9 \mathbf{i} \mathbf{b} z^3 \mathbf{k}^2 \mathbf{m} \mathbf{n} z \mathbf{r}^{3 + 3 \mathbf{n} z} + \mathbf{D} \mathbf{b} \phi^3 \mathbf{H}^2 \mathbf{m}^2 (-3 \mathbf{r}^2 + \mathbf{H}^2 (\mathbf{m}^2 + \mathbf{k}^2 \mathbf{r}^2)) + 3 \mathbf{i} \mathbf{b} z \mathbf{D} \mathbf{b} \phi^2 \\ & \quad \mathbf{m} \mathbf{n} z \mathbf{r}^{1 + \mathbf{n} z} (-3 \mathbf{r}^2 + \mathbf{H}^2 (\mathbf{m}^2 + \mathbf{k}^2 \mathbf{r}^2)) + 3 \mathbf{b} z^2 \mathbf{D} \mathbf{b} \phi \mathbf{r}^{2 \mathbf{n} z} (-3 \mathbf{m}^2 (4 + 3 \mathbf{n} z) \mathbf{r}^2 + \\ & \quad \mathbf{H}^2 (\mathbf{m}^2 + \mathbf{k}^2 \mathbf{r}^2) (\mathbf{m}^2 (2 + 3 \mathbf{n} z) + \mathbf{k}^2 (5 + 2 \mathbf{n} z) \mathbf{r}^2)) \big) + 9 \mathbf{r} (-6 \mathbf{i} \mathbf{b} z \mathbf{D} \mathbf{b} \phi \mathbf{k}^2 \\ & \quad \mathbf{m} \mathbf{r}^{3 + \mathbf{n} z} + 2 \mathbf{b} z^2 \mathbf{k}^2 \mathbf{r}^{2 + 2 \mathbf{n} z} (\mathbf{m}^2 + \mathbf{k}^2 \mathbf{r}^2) + \mathbf{D} \mathbf{b} \phi^2 \mathbf{m}^2 (-3 \mathbf{r}^2 + \mathbf{H}^2 (\mathbf{m}^2 + \mathbf{k}^2 \mathbf{r}^2)) \big) \\ & \quad \mathbf{c} [\mathbf{r}]^2 \Sigma' [\mathbf{r}] \big) \Omega' [\mathbf{r}] + 3 \mathbf{b} z^2 \mathbf{D} \mathbf{b} \phi^2 \mathbf{r}^{1 + 2 \mathbf{n} z} (-3 \mathbf{m}^2 \mathbf{r}^2 + \mathbf{H}^2 (\mathbf{m}^2 + \mathbf{k}^2 \mathbf{r}^2)^2) \Omega'' [\mathbf{r}] + \\ & 3 \mathbf{c} [\mathbf{r}] \Sigma [\mathbf{r}]^2 \big( 2 \mathbf{r} (-6 \mathbf{i} \mathbf{b} z \mathbf{D} \mathbf{b} \phi \mathbf{k}^2 \mathbf{m} \mathbf{r}^{3 + \mathbf{n} z} + 3 \mathbf{b} z^2 \mathbf{k}^2 \mathbf{r}^{2 + 2 \mathbf{n} z} (\mathbf{m}^2 + \mathbf{k}^2 \mathbf{r}^2) + \\ & \quad \mathbf{D} \mathbf{b} \phi^2 \mathbf{m}^2 (-3 \mathbf{r}^2 + \mathbf{H}^2 (\mathbf{m}^2 + \mathbf{k}^2 \mathbf{r}^2)) \big) \mathbf{c}' [\mathbf{r}] \Omega' [\mathbf{r}] + \mathbf{c} [\mathbf{r}] \big( (-3 \mathbf{i} \mathbf{b} z \mathbf{D} \mathbf{b} \phi \mathbf{k}^2 \mathbf{m} \\ & \quad (9 + \mathbf{n} z) \mathbf{r}^{3 + \mathbf{n} z} + 3 \mathbf{b} z^2 \mathbf{k}^2 \mathbf{r}^{2 + 2 \mathbf{n} z} (2 \mathbf{m}^2 (2 + \mathbf{n} z) + \mathbf{k}^2 (5 + 2 \mathbf{n} z) \mathbf{r}^2) + \\ & \quad \mathbf{D} \mathbf{b} \phi^2 \mathbf{m}^2 (-12 \mathbf{r}^2 + \mathbf{H}^2 (2 \mathbf{m}^2 + 5 \mathbf{k}^$$

$$\begin{aligned} S1 &= \left( m^2 r^2 \left( \dot{b} b z D b \phi k^2 r^{1+nz} \left( D b \phi^2 H^2 + 3 b z^2 r^{2+nz} \right) - m \left( 3 b z^2 k^2 r^{2+2nz} + D b \phi^2 \left( H^2 m^2 - 3 r^2 \right) \right) \sigma[r]^2 \Sigma[r] + \right. \right. \\ &\quad \left. \left. 3 m^3 r^2 \sigma[r]^4 \Sigma[r]^2 \right) \right) / \left( b z^2 D b \phi^2 r^{2+nz} \left( -3 m^2 r^2 + H^2 \left( m^2 + k^2 r^2 \right)^2 \right) - \right. \\ &\quad \left. m^2 r^2 \left( 3 b z^2 r^{2+nz} \left( m^2 + k^2 r^2 \right) + D b \phi^2 \left( -3 r^2 + H^2 \left( m^2 + k^2 r^2 \right) \right) \right) \sigma[r]^2 \Sigma[r] + \right. \\ &\quad \left. 3 m^4 r^4 \sigma[r]^4 \Sigma[r]^2 + c[r]^2 \Sigma[r] \left( -6 \dot{b} b z D b \phi k^2 m r^{3+nz} + 3 b z^2 k^2 r^{2+2nz} \left( m^2 + k^2 r^2 \right) + \right. \right. \\ &\quad \left. \left. D b \phi^2 m^2 \left( -3 r^2 + H^2 \left( m^2 + k^2 r^2 \right) \right) - 3 m^2 r^2 \left( m^2 + k^2 r^2 \right) \sigma[r]^2 \Sigma[r] \right) \right) \\ S0 &= \left( -3 b z^3 D b \phi^3 r^{1+3nz} \left( -3 m^2 r^2 + H^2 \left( m^2 + k^2 r^2 \right)^2 \right) \right. \\ &\quad \left. \left( -\dot{b} D b \phi^2 H^2 k^2 m r^3 - 3 \dot{b} b z^2 k^2 m r^{3+2nz} + b z D b \phi r^{nz} \left( -3 m^2 r^2 + H^2 \left( m^2 + k^2 r^2 \right)^2 \right) \right) \Sigma'[r] + \right. \\ &\quad \left. b z^2 D b \phi^2 r^{2+nz} \Sigma[r] \left( D b \phi^4 H^6 m^8 - 6 D b \phi^4 H^4 m^6 r^2 + 3 D b \phi^4 H^6 k^2 m^6 r^2 + 9 D b \phi^4 H^2 m^4 r^4 - \right. \right. \\ &\quad \left. \left. 9 D b \phi^4 H^4 k^2 m^4 r^4 + 3 D b \phi^4 H^6 k^4 m^4 r^4 - 3 D b \phi^4 H^4 k^4 m^2 r^6 + D b \phi^4 H^6 k^6 m^2 r^6 + \right. \right. \\ &\quad \left. \left. 3 b z^2 D b \phi^2 H^4 m^8 n z r^{2+nz} + 9 \dot{b} b z D b \phi^3 H^4 k^2 m^5 r^{3+nz} - 3 \dot{b} b z D b \phi^3 H^4 k^2 m^5 n z r^{3+nz} - \right. \right. \end{aligned}$$



$$\begin{aligned}
& 9 \, i \, b z \, D b \phi^3 \, H^2 \, k^2 \, m^3 \, r^{5+n z} + 6 \, i \, b z \, D b \phi^3 \, H^4 \, k^4 \, m^3 \, r^{5+n z} + 9 \, i \, b z \, D b \phi^3 \, H^2 \, k^2 \, m^3 \, n z \, r^{5+n z} - \\
& 6 \, i \, b z \, D b \phi^3 \, H^4 \, k^4 \, m^3 \, n z \, r^{5+n z} - 3 \, i \, b z \, D b \phi^3 \, H^4 \, k^6 \, m \, r^{7+n z} - 3 \, i \, b z \, D b \phi^3 \, H^4 \, k^6 \, m \, n z \, r^{7+n z} - \\
& 3 \, b z^2 \, D b \phi^2 \, H^4 \, k^2 \, m^6 \, r^{2+2 \, n z} - 18 \, b z^2 \, D b \phi^2 \, H^2 \, m^6 \, n z \, r^{2+2 \, n z} + 9 \, b z^2 \, D b \phi^2 \, H^4 \, k^2 \, m^6 \, n z \, r^{2+2 \, n z} + \\
& 9 \, b z^2 \, D b \phi^2 \, H^2 \, k^2 \, m^4 \, r^{4+2 \, n z} - 9 \, b z^2 \, D b \phi^2 \, H^4 \, k^4 \, m^4 \, r^{4+2 \, n z} + 27 \, b z^2 \, D b \phi^2 \, m^4 \, n z \, r^{4+2 \, n z} - \\
& 27 \, b z^2 \, D b \phi^2 \, H^2 \, k^2 \, m^4 \, n z \, r^{4+2 \, n z} + 9 \, b z^2 \, D b \phi^2 \, H^4 \, k^4 \, m^4 \, n z \, r^{4+2 \, n z} + 9 \, b z^2 \, D b \phi^2 \, H^2 \, k^4 \, m^2 \, r^{6+2 \, n z} - \\
& 9 \, b z^2 \, D b \phi^2 \, H^4 \, k^6 \, m^2 \, r^{6+2 \, n z} - 9 \, b z^2 \, D b \phi^2 \, H^2 \, k^4 \, m^2 \, n z \, r^{6+2 \, n z} + 3 \, b z^2 \, D b \phi^2 \, H^4 \, k^6 \, m^2 \, n z \, r^{6+2 \, n z} - \\
& 3 \, b z^2 \, D b \phi^2 \, H^4 \, k^8 \, r^{8+2 \, n z} + 27 \, i \, b z^3 \, D b \phi \, H^2 \, k^2 \, m^5 \, r^{3+3 \, n z} - 9 \, i \, b z^3 \, D b \phi \, H^2 \, k^2 \, m^5 \, n z \, r^{3+3 \, n z} - \\
& 27 \, i \, b z^3 \, D b \phi \, k^2 \, m^3 \, r^{5+3 \, n z} + 18 \, i \, b z^3 \, D b \phi \, H^2 \, k^4 \, m^3 \, r^{5+3 \, n z} + 27 \, i \, b z^3 \, D b \phi \, k^2 \, m^3 \, n z \, r^{5+3 \, n z} - \\
& 18 \, i \, b z^3 \, D b \phi \, H^2 \, k^4 \, m^3 \, n z \, r^{5+3 \, n z} - 9 \, i \, b z^3 \, D b \phi \, H^2 \, k^6 \, m \, r^{7+3 \, n z} - 9 \, i \, b z^3 \, D b \phi \, H^2 \, k^6 \, m \, n z \, r^{7+3 \, n z} + \\
& 9 \, b z^4 \, H^2 \, k^2 \, m^6 \, n z \, r^{2+4 \, n z} - 27 \, b z^4 \, k^2 \, m^4 \, n z \, r^{4+4 \, n z} + 27 \, b z^4 \, H^2 \, k^4 \, m^4 \, n z \, r^{4+4 \, n z} - 27 \, b z^4 \, k^4 \, m^2 \, n z \, r^{6+4 \, n z} + \\
& 27 \, b z^4 \, H^2 \, k^6 \, m^2 \, n z \, r^{6+4 \, n z} + 9 \, b z^4 \, H^2 \, k^8 \, n z \, r^{8+4 \, n z} - 3 \, r \left( -3 \, m^2 \, r^2 + H^2 \left( m^2 + k^2 \, r^2 \right)^2 \right) \\
& \left( -6 \, i \, b z \, D b \phi \, k^2 \, m \, r^{3+n z} + 3 \, b z^2 \, k^2 \, r^{2+2 \, n z} \left( m^2 + k^2 \, r^2 \right) + D b \phi^2 \, m^2 \left( -3 \, r^2 + H^2 \left( m^2 + k^2 \, r^2 \right)^2 \right) \right) c[r]^2 \\
& \Sigma'[r] + 6 \, m^2 \, r^3 \left( D b \phi^2 \, H^2 \, k^2 \, r^2 + 3 \, b z^2 \, m^2 \, r^{2 \, n z} \right) \left( -3 \, m^2 \, r^2 + H^2 \left( m^2 + k^2 \, r^2 \right)^2 \right) \sigma[r]^2 \Sigma'[r] + \\
& 54 \, m^6 \, r^6 \, \sigma[r]^5 \Sigma[r]^5 \left( m^2 \, r^2 \, \sigma[r]^2 \Omega[r] + r \left( m^2 + k^2 \, r^2 \right) c[r] \, \sigma[r] \, c'[r] - \right. \\
& \left. c[r]^2 \left( m^2 \, \sigma[r] + \left( m^2 + k^2 \, r^2 \right) \left( \Omega[r] + r \, \Omega'[r] \right) \right) \right) - \\
& 9 \, m^3 \, r^4 \, \sigma[r]^3 \Sigma[r]^4 \left( 2 \, m \, r \left( -6 \, i \, b z \, D b \phi \, k^2 \, m \, r^{3+n z} + 6 \, b z^2 \, k^2 \, r^{2+2 \, n z} \left( m^2 + k^2 \, r^2 \right) + \right. \right. \\
& \left. \left. D b \phi^2 \left( -3 \, r^2 \left( 2 \, m^2 + k^2 \, r^2 \right) + 2 \, H^2 \left( m^4 + k^2 \, m^2 \, r^2 \right) \right) \right) c[r] \, \sigma[r] \, c'[r] + \right. \\
& \left. m^2 \, r^2 \, \sigma[r]^2 \left( m \left( D b \phi^2 \, H^2 \left( m^2 - k^2 \, r^2 \right) - 3 \, b z^2 \, r^{2 \, n z} \left( m^2 \left( -2 + n z \right) - k^2 \, n z \, r^2 \right) \right) \sigma[r] + \right. \right. \\
& \left. \left. 2 \left( \left( -3 \, i \, b z \, D b \phi \, k^2 \, r^{3+n z} + 3 \, b z^2 \, m \, r^{2 \, n z} \left( m^2 + k^2 \, r^2 \right) + 2 \, D b \phi^2 \, m \left( -3 \, r^2 + H^2 \left( m^2 + k^2 \, r^2 \right)^2 \right) \right) \Omega[r] + \right. \right. \right. \\
& \left. \left. m \, r \left( D b \phi^2 \, H^2 \, k^2 \, r^2 + 3 \, b z^2 \, m^2 \, r^{2 \, n z} \right) \Omega'[r] \right) - c[r]^2 \left( m \left( 6 \, i \, b z \, D b \phi \, k^2 \, m \left( -1 + n z \right) \, r^{3+n z} + \right. \right. \right. \\
& \left. \left. \left. 3 \, b z^2 \, r^{2 \, n z} \left( m^4 \, n z + 2 \, k^2 \, m^2 \left( 2 + n z \right) \, r^2 + k^4 \, n z \, r^4 \right) + D b \phi^2 \left( -12 \, m^2 \, r^2 + H^2 \left( 5 \, m^4 - k^4 \, r^4 \right) \right) \right) \right) \right) \\
& \sigma[r] + 2 \left( \left( 3 \, b z^2 \, k^2 \, m \, r^{2+2 \, n z} \left( m^2 + k^2 \, r^2 \right) - 3 \, i \, b z \, D b \phi \, k^2 \, r^{3+n z} \left( 3 \, m^2 + k^2 \, r^2 \right) + \right. \right. \\
& \left. \left. D b \phi^2 \, m \left( 2 \, m^2 + k^2 \, r^2 \right) \left( -3 \, r^2 + H^2 \left( m^2 + k^2 \, r^2 \right)^2 \right) \right) \Omega[r] + 2 \, m \, r \left( -6 \, i \, b z \, D b \phi \, k^2 \, m \, r^{3+n z} + \right. \right. \\
& \left. \left. 3 \, b z^2 \, k^2 \, r^{2+2 \, n z} \left( m^2 + k^2 \, r^2 \right) + D b \phi^2 \, m^2 \left( -3 \, r^2 + H^2 \left( m^2 + k^2 \, r^2 \right)^2 \right) \right) \Omega'[r] \right) - \\
& 3 \, m \, r^2 \, \sigma[r] \, \Sigma[r]^3 \left( -2 \, m \, r \left( -9 \, i \, b z^3 \, D b \phi \, k^2 \, m \, r^{3+3 \, n z} \left( -m^2 + k^2 \, r^2 \right) + 9 \, b z^4 \, k^4 \, r^{4+4 \, n z} \left( m^2 + k^2 \, r^2 \right) + 3 \right. \right. \\
& \left. \left. i \, b z \, D b \phi^3 \, k^2 \, m \, r^{3+n z} \left( 6 \, r^2 + H^2 \left( -m^2 + k^2 \, r^2 \right) \right) + D b \phi^4 \, m^2 \left( H^2 \, m^2 - 3 \, r^2 \right) \left( -3 \, r^2 + H^2 \left( m^2 + k^2 \, r^2 \right)^2 \right) \right) + \right. \\
& \left. 3 \, b z^2 \, D b \phi^2 \, k^2 \, r^{2+2 \, n z} \left( -3 \, r^2 \left( 2 \, m^2 + k^2 \, r^2 \right) + 2 \, H^2 \left( m^4 + k^2 \, m^2 \, r^2 \right) \right) \right) c[r] \, \sigma[r] \, c'[r] + \\
& m^2 \, r^2 \, \sigma[r]^2 \left( m \left( -3 \, i \, b z \, D b \phi^3 \, H^2 \, k^2 \, m \left( -1 + n z \right) \, r^{3+n z} - 9 \, i \, b z^3 \, D b \phi \, k^2 \, m \left( -1 + n z \right) \, r^{3+3 \, n z} - \right. \right. \\
& \left. \left. 9 \, b z^4 \, r^4 \, n z \left( m^4 \, n z + k^2 \, m^2 \left( 2 + 3 \, n z \right) \, r^2 + 2 \, k^4 \, n z \, r^4 \right) + 3 \, b z^2 \, D b \phi^2 \, r^{2 \, n z} \right. \right. \\
& \left. \left. \left( H^2 \left( m^2 + k^2 \, r^2 \right) \left( m^2 \left( -5 + 2 \, n z \right) - k^2 \left( -2 + n z \right) \, r^2 \right) + 3 \, r^2 \left( -2 \, m^2 \left( -2 + n z \right) + k^2 \, n z \, r^2 \right) \right) \right) + \right. \\
& \left. D b \phi^4 \, H^2 \left( 6 \, m^2 \, r^2 - 3 \, k^2 \, r^4 + H^2 \left( -2 \, m^4 + k^2 \, m^2 \, r^2 + k^4 \, r^4 \right) \right) \right) \sigma[r] - \\
& 2 \, D b \phi \left( \left( -9 \, i \, b z^3 \, k^2 \, r^{3+3 \, n z} \left( m^2 + k^2 \, r^2 \right) - 3 \, i \, b z \, D b \phi^2 \, k^2 \, r^{3+n z} \left( -3 \, r^2 + H^2 \left( m^2 + k^2 \, r^2 \right)^2 \right) \right) + \right. \\
& \left. D b \phi^3 \, m \left( -3 \, r^2 + H^2 \left( m^2 + k^2 \, r^2 \right)^2 \right) + 3 \, b z^2 \, D b \phi \, m \, r^{2 \, n z} \right. \\
& \left. \left( 2 \, H^2 \left( m^2 + k^2 \, r^2 \right)^2 - 3 \, r^2 \left( 2 \, m^2 + k^2 \, r^2 \right) \right) \right) \Omega[r] + 6 \, b z \, m \, r^{1+n z} \left( -i \, D b \phi^2 \, H^2 \, k^2 \, m \, r^3 - \right. \\
& \left. 3 \, i \, b z^2 \, k^2 \, m \, r^{3+2 \, n z} + b z \, D b \phi \, r^{n z} \left( -3 \, m^2 \, r^2 + H^2 \left( m^2 + k^2 \, r^2 \right)^2 \right) \right) \Omega'[r] + \\
& c[r]^2 \left( m \left( -9 \, i \, b z^3 \, D b \phi \, k^2 \, m \, r^{3+3 \, n z} \left( m^2 \left( -1 + n z \right) + 3 \, k^2 \left( 1 + n z \right) \, r^2 \right) + 18 \, b z^4 \, k^2 \, r^{2+4 \, n z} \left( m^4 \, n z + \right. \right. \right. \\
& \left. \left. k^2 \, m^2 \left( 1 + 2 \, n z \right) \, r^2 + k^4 \, n z \, r^4 \right) + 2 \, D b \phi^4 \, m^2 \left( H^2 \, m^2 - 3 \, r^2 \right) \left( -3 \, r^2 + H^2 \left( 2 \, m^2 + k^2 \, r^2 \right) \right) + \right. \\
& \left. 3 \, i \, b z \, D b \phi^3 \, k^2 \, m \, r^{3+n z} \left( -6 \left( -1 + n z \right) \, r^2 + H^2 \left( m^2 \left( 1 + 3 \, n z \right) + k^2 \left( 1 + n z \right) \, r^2 \right) \right) + \right. \\
& \left. 6 \, b z^2 \, D b \phi^2 \, r^{2 \, n z} \left( -3 \, r^2 \left( m^4 \, n z + k^2 \, m^2 \left( 2 + n z \right) \, r^2 - k^4 \, n z \, r^4 \right) + \right. \right. \\
& \left. \left. H^2 \left( m^6 \, n z + 2 \, k^2 \, m^4 \left( 1 + n z \right) \, r^2 + k^4 \, m^2 \left( -1 + n z \right) \, r^4 - k^6 \, r^6 \right) \right) \right) \sigma[r] + \\
& 3 \, m^3 \, r^3 \left( 6 \, i \, b z \, D b \phi \, k^2 \, m \, r^{3+n z} + 3 \, b z^2 \, m^2 \, r^{2 \, n z} \left( m^2 + k^2 \, r^2 \right) + D b \phi^2 \, k^2 \, r^2 \left( -3 \, r^2 + H^2 \left( m^2 + k^2 \, r^2 \right)^2 \right) \right) \\
& \sigma[r]^3 \Sigma'[r] + 2 \left( D b \phi \left( -9 \, i \, b z^3 \, k^4 \, r^{5+3 \, n z} \left( m^2 + k^2 \, r^2 \right) - 9 \, i \, b z \, D b \phi^2 \, k^2 \, m^2 \right. \right. \\
& \left. \left. r^{3+n z} \left( -3 \, r^2 + H^2 \left( m^2 + k^2 \, r^2 \right)^2 \right) + D b \phi^3 \, m^3 \left( -3 \, r^2 + H^2 \left( m^2 + k^2 \, r^2 \right)^2 \right) \right)^2 + \\
& 3 \, b z^2 \, D b \phi \, k^2 \, m \, r^{2+2 \, n z} \left( H^2 \left( m^2 + k^2 \, r^2 \right)^2 - 3 \, r^2 \left( m^2 + 3 \, k^2 \, r^2 \right) \right) \Omega[r] + \\
& m \, r \left( 9 \, b z^4 \, k^4 \, r^{4+4 \, n z} \left( m^2 + k^2 \, r^2 \right) - 9 \, i \, b z^3 \, D b \phi \, k^2 \, m \, r^{3+3 \, n z} \left( m^2 + 3 \, k^2 \, r^2 \right) + D b \phi^4 \, m^2 \left( H^2 \, m^2 - \right. \right. \\
& \left. \left. 3 \, r^2 \right) \left( -3 \, r^2 + H^2 \left( m^2 + k^2 \, r^2 \right)^2 \right) - 3 \, i \, b z \, D b \phi^3 \, k^2 \, m \, r^{3+n z} \left( -6 \, r^2 + H^2 \left( 3 \, m^2 + k^2 \, r^2 \right) \right) + \right. \\
& \left. 3 \, b z^2 \, D b \phi^2 \, k^2 \, r^{2+2 \, n z} \left( -3 \, r^2 \left( 2 \, m^2 + k^2 \, r^2 \right) + 2 \, H^2 \left( m^4 + k^2 \, m^2 \, r^2 \right) \right) \right) \Omega'[r] \right) +
\end{aligned}$$

$$\begin{aligned}
& \Sigma[r]^2 \left( -6 \, i \, b z \, D b \phi \, k^2 \, m \, r^{4+n z} \left( D b \phi^2 \, H^2 + 3 \, b z^2 \, r^{2 n z} \right) \left( -6 \, i \, b z \, D b \phi \, k^2 \, m \, r^{3+n z} + \right. \right. \\
& \quad \left. \left. 3 \, b z^2 \, k^2 \, r^{2+2 n z} \left( m^2 + k^2 \, r^2 \right) + D b \phi^2 \, m^2 \left( -3 \, r^2 + H^2 \left( m^2 + k^2 \, r^2 \right) \right) \right) \right) c[r] \, c'[r] + c[r]^2 \\
& \quad \left( 27 \, b z^6 \, k^4 \, n z \, r^{4+6 n z} \left( m^2 + k^2 \, r^2 \right)^2 - 27 \, i \, b z^5 \, D b \phi \, k^4 \, m \, r^{5+5 n z} \left( m^2 \left( -1 + 3 \, n z \right) + k^2 \left( 1 + 3 \, n z \right) \, r^2 \right) + \right. \\
& \quad \left. 3 \, b z^2 \, D b \phi^4 \, m^4 \, n z \, r^{2 n z} \left( -3 \, r^2 + H^2 \left( m^2 + k^2 \, r^2 \right) \right)^2 + D b \phi^6 \, m^4 \left( -3 \, H \, r^2 + H^3 \left( m^2 + k^2 \, r^2 \right) \right)^2 - \right. \\
& \quad \left. 9 \, b z^4 \, D b \phi^2 \, k^2 \, r^{2+4 n z} \left( m^2 + k^2 \, r^2 \right) \left( 6 \, m^2 \, n z \, r^2 - H^2 \left( 2 \, m^2 \, n z - k^2 \, r^2 \right) \left( m^2 + k^2 \, r^2 \right) \right) - \right. \\
& \quad \left. 9 \, i \, b z^3 \, D b \phi^3 \, k^2 \, m \, r^{3+3 n z} \left( -3 \, m^2 \left( -1 + n z \right) \, r^2 + H^2 \left( m^2 + k^2 \, r^2 \right) \left( m^2 \left( -3 + n z \right) + k^2 \left( -1 + n z \right) \, r^2 \right) \right) + \right. \\
& \quad \left. 3 \, i \, b z \, D b \phi^5 \, H^2 \, k^2 \, m^3 \, r^{3+n z} \left( -3 \left( -1 + n z \right) \, r^2 + H^2 \left( m^2 \left( 1 + n z \right) + k^2 \left( -1 + n z \right) \, r^2 \right) \right) + \right. \\
& \quad \left. 3 \, m^2 \, r^3 \left( -3 \, i \, b z \, D b \phi^3 \, H^2 \, k^2 \, m \, r^{3+n z} \left( -m^2 + k^2 \, r^2 \right) + 9 \, i \, b z^3 \, D b \phi \, k^2 \, m \, r^{3+3 n z} \left( -m^2 + k^2 \, r^2 \right) + \right. \right. \\
& \quad \left. \left. 9 \, b z^4 \, k^2 \, m^2 \, r^{2+4 n z} \left( m^2 + k^2 \, r^2 \right) + D b \phi^4 \, H^2 \, k^2 \, m^2 \, r^2 \left( -3 \, r^2 + H^2 \left( m^2 + k^2 \, r^2 \right) \right) + 3 \, b z^2 \, D b \phi^2 \right. \right. \\
& \quad \left. \left. r^{2 n z} \left( -3 \, m^2 \, r^2 \left( 2 \, m^2 + k^2 \, r^2 \right) + 2 \, H^2 \left( m^6 + 2 \, k^2 \, m^4 \, r^2 + 2 \, k^4 \, m^2 \, r^4 + k^6 \, r^6 \right) \right) \right) \right) \sigma[r]^2 \, \Sigma'[r] \right) - \\
& \quad m \, r^2 \, \sigma[r] \left( m \left( 27 \, b z^6 \, k^2 \, n z \, r^{2+6 n z} \left( m^2 + k^2 \, r^2 \right)^2 - 27 \, i \, b z^5 \, D b \phi \, k^2 \, m \, r^{3+5 n z} \right. \right. \\
& \quad \left. \left( m^2 \left( -1 + n z \right) + k^2 \left( 1 + n z \right) \, r^2 \right) - 9 \, i \, b z^3 \, D b \phi^3 \, k^2 \, m \, r^{3+3 n z} \right. \\
& \quad \left. \left( 3 \left( -1 + n z \right) \, r^2 - 2 \, H^2 \left( m^2 - k^2 \, r^2 \right) \right) + D b \phi^6 \, H^2 \, m^2 \left( -3 \, r^2 + H^2 \left( m^2 + k^2 \, r^2 \right) \right)^2 + \right. \\
& \quad \left. 3 \, i \, b z \, D b \phi^5 \, H^2 \, k^2 \, m \, r^{3+n z} \left( -3 \left( -1 + n z \right) \, r^2 + H^2 \left( m^2 \left( 1 + n z \right) + k^2 \left( -1 + n z \right) \, r^2 \right) \right) - 3 \, b z^2 \right. \\
& \quad \left. D b \phi^4 \, r^{2 n z} \left( 9 \, m^2 \left( -2 + n z \right) \, r^4 + H^4 \left( m^2 + k^2 \, r^2 \right) \left( m^4 \left( -4 + n z \right) + k^2 \, m^2 \left( 2 + n z \right) \, r^2 + 2 \, k^4 \, r^4 \right) - \right. \right. \\
& \quad \left. \left. 3 \, H^2 \, r^2 \left( 2 \, m^4 \left( -3 + n z \right) + k^2 \, m^2 \left( -3 + 2 \, n z \right) \, r^2 + k^4 \left( 1 + 2 \, n z \right) \, r^4 \right) \right) + \right. \\
& \quad \left. 9 \, b z^4 \, D b \phi^2 \, r^{4 n z} \left( H^2 \left( m^2 + k^2 \, r^2 \right) \left( 2 \, m^4 \, n z + k^2 \, m^2 \left( 3 + 4 \, n z \right) \, r^2 + k^4 \left( -1 + 2 \, n z \right) \, r^4 \right) - \right. \right. \\
& \quad \left. \left. 3 \left( 2 \, m^4 \, n z \, r^2 + k^2 \, m^2 \left( 2 + 3 \, n z \right) \, r^4 + k^4 \, n z \, r^6 \right) \right) \right) \sigma[r] + \right. \\
& \quad \left. 3 \, m^3 \, r^3 \left( 3 \, i \, b z \, D b \phi^3 \, H^2 \, k^2 \, m \, r^{3+n z} + 9 \, i \, b z^3 \, D b \phi \, k^2 \, m \, r^{3+3 n z} + 9 \, b z^4 \, m^2 \, r^{4 n z} \left( m^2 + k^2 \, r^2 \right) + \right. \right. \\
& \quad \left. \left. D b \phi^4 \, H^2 \, k^2 \, r^2 \left( -3 \, r^2 + H^2 \left( m^2 + k^2 \, r^2 \right) \right) \right) \right) \sigma[r]^3 \, \Sigma'[r] + \right. \\
& \quad \left. 6 \, b z \, D b \phi \, r^{n z} \left( b z \, D b \phi^2 \, r^{n z} \left( -3 \, m^2 \, r^2 + H^2 \left( m^2 + k^2 \, r^2 \right) \right)^2 \left( -3 \, i \, b z \, k^2 \, r^{3+n z} + \right. \right. \right. \\
& \quad \left. \left. D b \phi \, m \left( -3 \, r^2 + H^2 \left( m^2 + k^2 \, r^2 \right) \right) \right) \Omega[r] + m \, r \left( -9 \, i \, b z^4 \, k^2 \, m \, r^{3+4 n z} \left( m^2 + k^2 \, r^2 \right) - \right. \right. \\
& \quad \left. \left. i \, D b \phi^4 \, H^2 \, k^2 \, m \, r^3 \left( -3 \, r^2 + H^2 \left( m^2 + k^2 \, r^2 \right) \right) - 3 \, i \, b z^2 \, D b \phi^2 \, k^2 \, m \, r^{3+2 n z} \right. \right. \\
& \quad \left. \left. \left( -3 \, r^2 + 2 \, H^2 \left( m^2 + k^2 \, r^2 \right) \right) + 3 \, b z^3 \, D b \phi \, k^2 \, r^{2+3 n z} \left( -3 \, m^2 \, r^2 + H^2 \left( m^2 + k^2 \, r^2 \right) \right)^2 + b z \right. \right. \\
& \quad \left. \left. D b \phi^3 \, r^{n z} \left( 9 \, m^2 \, r^4 + H^4 \left( m^3 + k^2 \, m \, r^2 \right) \right)^2 - 3 \, H^2 \left( 2 \, m^4 \, r^2 + 2 \, k^2 \, m^2 \, r^4 + k^4 \, r^6 \right) \right) \right) \Omega'[r] \right) \right) \right) / \\
& \quad \left( 3 \, r \, \Sigma[r] \left( b z^2 \, D b \phi^2 \, r^{2 n z} \left( -3 \, m^2 \, r^2 + H^2 \left( m^2 + k^2 \, r^2 \right) \right)^2 - m^2 \, r^2 \left( 3 \, b z^2 \, r^{2 n z} \left( m^2 + k^2 \, r^2 \right) + \right. \right. \right. \\
& \quad \left. \left. D b \phi^2 \left( -3 \, r^2 + H^2 \left( m^2 + k^2 \, r^2 \right) \right) \right) \right) \sigma[r]^2 \, \Sigma[r] + 3 \, m^4 \, r^4 \, \sigma[r]^4 \, \Sigma[r]^2 + \right. \\
& \quad \left. c[r]^2 \, \Sigma[r] \left( -6 \, i \, b z \, D b \phi \, k^2 \, m \, r^{3+n z} + 3 \, b z^2 \, k^2 \, r^{2+2 n z} \left( m^2 + k^2 \, r^2 \right) + \right. \right. \\
& \quad \left. \left. D b \phi^2 \, m^2 \left( -3 \, r^2 + H^2 \left( m^2 + k^2 \, r^2 \right) \right) - 3 \, m^2 \, r^2 \left( m^2 + k^2 \, r^2 \right) \sigma[r]^2 \, \Sigma[r] \right) \right)^2 \right)
\end{aligned}$$

(\*end of file\*)
